# Supplementary material for: Post-Processed Posteriors for Banded Covariances
Source: arXiv:2011.12627 ancillary file (2020-11-25)
Supplement: Supplementary file 1 [file cov-ppp-supp.pdf]

# Supplementary Material for "Post-Processed Posteriors for Banded Covariances"


Kwangmin Lee[1], Kyoungjae Lee[2], and Jaeyong Lee[1]

[1]*Department of Statistics, Seoul National University*

[2]*Department Statistics, Inha University*


November 25, 2020

In the supplementary material, we represent futher materials. In Section 1, we show the result of minimax convergence rate for bandable covariance case. In Section 2, we represent more simulation results. In Section 3, we give an example of application to Linear Discriminant Analysis. Finally, in Section 4, we prove lemmas and theorems of the main paper.

## 1 Bandable covariance case

In this section, we show that the banding post-processed posterior is nearly optimal in the minimax sense for the class of bandable covariance matrices. Cai and Zhou (2010) considered the following clasee of bandable covariance matrices,

$$\begin{aligned}\mathcal{F}_\alpha &:= \mathcal{F}_\alpha(M, M_0, M_1)\\ &= \Big\{\Sigma = (\sigma_{ij}) \in \mathcal{C}_p : \sum_{(i,j):|i-j|\geq k} |\sigma_{ij}| \leq Mk^{-\alpha}, \forall k \geq 1, \lambda_{\max}(\Sigma) \leq M_0, \lambda_{\min}(\Sigma) \geq M_1\Big\},\end{aligned} \quad (1)$$

where $\alpha, M > 0$ and $0 < M_1 < M_0$. In this subsection, we assume $\Sigma_0 \in \mathcal{F}_\alpha$.

The following theorems show the convergence rate of the banding post-processed posterior, and the minimax lower bound for the bandable covariances.

**Theorem 1.1** *Let prior* $\pi^i$ *of* $\Sigma$ *be* $IW_p(A_n, \nu_n)$*. If* $A_n \in \mathcal{B}_{p,k}$ *and* $n/4 \geq (M_0^{1/2} M_1^{-1} \log p) \vee k \vee ||A_n|| \vee (\nu_n - 2p)$*, then*

$$\sup_{\Sigma_0 \in \mathcal{F}_\alpha} E_{\Sigma_0}\{E^{\pi^i}(||B_k^{(\epsilon_n)}(\Sigma) - \Sigma_0||^2 \mid \mathbb{X}_n)\} \ \leq \ C(\log k)^2 \frac{\log p + k}{n} + k^{-2\alpha},$$

*where* $\epsilon_n^2 = O\{(\log k)^2 (k + \log p)/n\}$*, and* $C$ *depends on* $M$*,* $M_0$ *and* $M_1$*.*

**Theorem 1.2** *If* $n \geq [2\min\{(M_0 - M_1)^2, 1\}\log p] \vee 2^{2\alpha/(2\alpha+1)}$*,*

$$\inf_{(\pi,f)\in\Pi^*} \sup_{\Sigma_0 \in \mathcal{F}_\alpha} E_{\Sigma_0} E^{\pi}\Big\{||f(\Sigma) - \Sigma_0||^2 \mid \mathbb{X}_n\Big\} \ \geq \ C \min\Big\{n^{-2\alpha/(2\alpha+1)} + \frac{\log p}{n}, \frac{p}{n}\Big\},$$

*where* $C$ *depends on* $M$*,* $M_0$ *and* $M_1$*.*

If we choose $k = n^{1/(2\alpha+1)}$ in the banding post-processed posterior, the convergence rate of the banding post-processed posterior in Theorem 1.1 is

$$C \min\Big\{(\log k)^2 \Big(n^{-2\alpha/(2\alpha+1)} + \frac{\log p}{n}\Big) + n^{-2\alpha/(2\alpha+1)}, \frac{p}{n}\Big\}.$$

Thus, the maximum risk in Theorem 1.1 is minimax optimal up to a factor of $(\log k)^2$. Cai and Zhou (2010) showed that the lower bound in Theorem 1.2 is the optimal minimax rate for estimators.

When $p \lesssim n^{1/(2\alpha+1)}$, the lower bounds in Theorem 1.2 is $p/n$, which is the optimal rate for unconstrained covariances (Lee and Lee; 2018). It means that $p \lesssim n^{1/(2\alpha+1)}$ can be roughly considered as a fixed dimensional case. In addition to $p \lesssim n^{1/(2\alpha+1)}$, if $[k^{2\alpha}\{p - (\log k)^2\}(\log p + k)] \lesssim n$, the banding post-processed posterior satisfies this optimal minimax rate.

It is somewhat surprising that the banding post-processed posterior is nearly minimax optimal rate because it was believed that the banding estimator gives the sub-optimal

convergence rate (Bickel and Levina; 2008) for bandable covariance matrices. Theorem 1.3 states that the banding estimator has the same convergence rate as the banding post-processed posterior.

**Theorem 1.3** *Suppose $X_1, \ldots, X_n$ are independent and identically distributed sample from the $N_p(0, \Sigma_0)$ and $S_n = n^{-1} \sum_{i=1}^{n} X_i X_i^T$. Then for all sufficiently large $n$,*

$$\sup_{\Sigma_0 \in \mathcal{F}_\alpha} E(||B_k(S_n) - \Sigma_0||^2) \leq C\Big\{(\log k)^2 \frac{\log p + k}{n} + k^{-2\alpha}\Big\},$$

*for some constant $C$.*

# 2 More simulation results

## 2.1 bandable covariance case

We consider a bandable covariance $\Sigma_0^{(4)}$. Let $\Sigma_0^{(4)*} = (\sigma_{0,ij}^{(4)})_{p \times p}$, where

$$\sigma_{0,ij}^{(4)} = \begin{cases} 1, & 1 \leq i = j \leq p \\ \rho |i-j|^{-(\alpha+1)}, & 1 \leq i \neq j \leq p, \end{cases}$$

$\rho = 0.6$ and $\alpha = 0.1$. Then we set $\Sigma_0^{(4)} = \Sigma_0^{(4)*} + [0.5 - \{\lambda_{min}(\Sigma_0^{(4)*}) \wedge 0\}]I_p$, which guarantees the minimum eigenvalue of $\Sigma^{(4)}$ to be 0.5. The true covariance matrice with $p = 100$ is described in Figure 1. Because there is no true bandwidth $k_0$ of the bandable covariance, we report the error of each method for various values of bandwidths in Figure 2. The post-processed posterior can be compatible with the banded sample covariance and iterative conditional fitting, and they has a smaller error in all the values of $k$ than the others.

## 2.2 Choice of the bandwidth

When the true bandwidth $k_0$ is unknown, we choose the bandwidth by the Bayesian leave-one-out cross-validation method as (7). However, for G-inverse Wishart and Wishart for

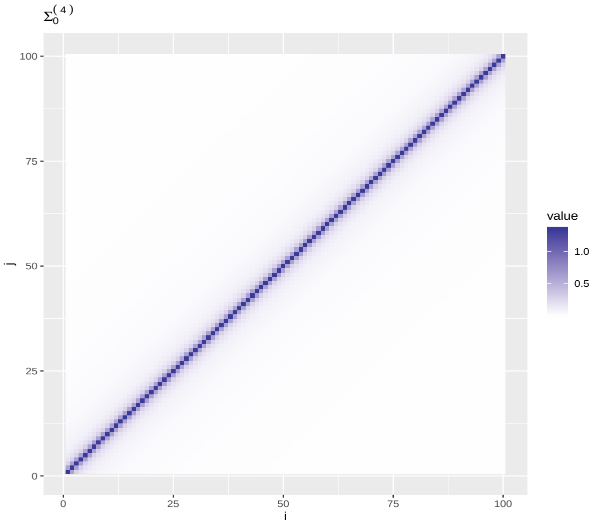


Figure 1: Visualization of the true bandable covariance.

covariance graph methods, since the normalization constants of the posterior distributions do not have closed forms, it is hard to calculate $\hat{R}(k)$. Thus, we omit those methods in the simulation for unknown bandwidth. For the frequentist methods, we use the leave-one-out cross-validation as we did in choosing $\epsilon_n$ for the frequentist methods. Due to the large computing time of the maximum likelihood estimator method, we omit this in the simulation.

Table 1 shows the error of estimators based on the selected bandwidths, which confirms that the post-processed posterior gives smaller errors for all settings.

# 3 Application to recognition of gestures

A covariance estimator can be used in the Linear discriminant analysis problem. In this section, we applied the post-processed posterior to analyze a data set (UWaveGesture-LibraryAll) in the University of East Anglia (UEA) and the University of California, Riverside (UCR) Time Series Classification Repository. The goal of the analysis is classification of eight gestures in Table 2 Liu et al. (2009). The data set consists of 896 training data and 3582 test data, and each observation represents one of eight simple gestures.

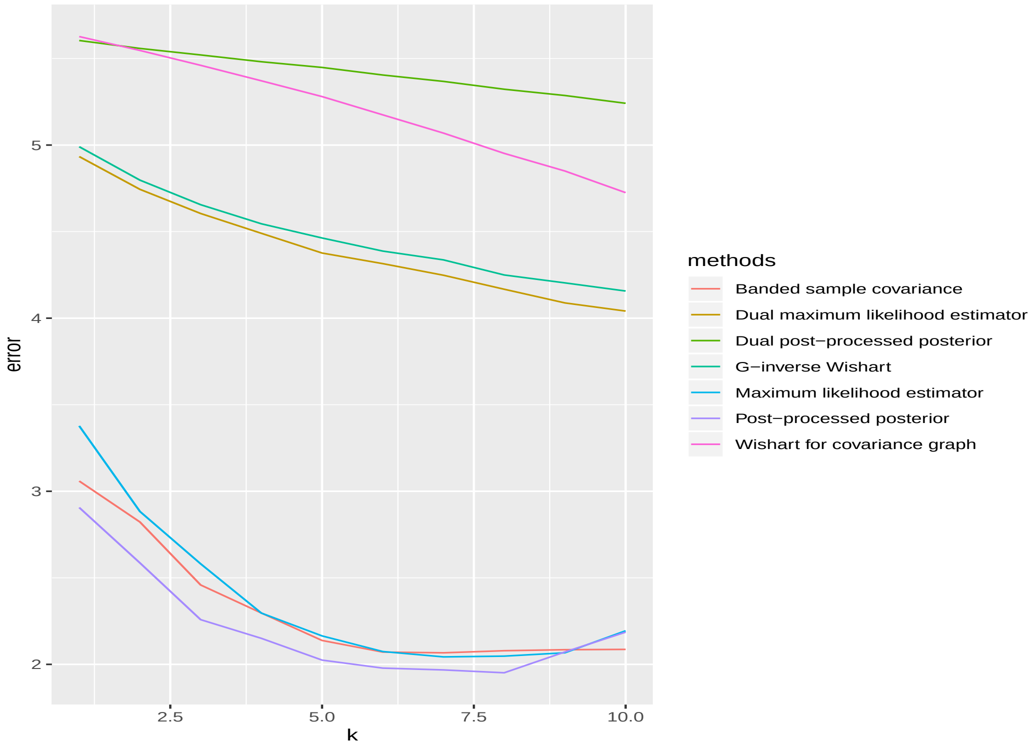


Figure 2: Errors of point estimators for the bandable covariance $\Sigma_0^{(4)}$ when $n = 100$ and $p = 100$. The errors are calculated with various bandwidths from 1 to 10. The $x$-axis represents the bandwidth parameter used for estimation and the $y$-axis represents the spectral norm between the true covariance and the estimated covariance.

Table 1: Errors of point estimators for banded covariances $\Sigma_0^{(1)}$, $\Sigma_0^{(2)}$, $\Sigma_0^{(3)}$ and $\Sigma_0^{(4)}$ with estimated bandwidths. Error is defined as the spectral norm of the difference between the true value and the point estimator.

| | $n = 50$ | | | | $n = 100$ | | | |
|---|---|---|---|---|---|---|---|---|
| | $\Sigma_0^{(1)}$ | $\Sigma_0^{(2)}$ | $\Sigma_0^{(3)}$ | $\Sigma_0^{(4)}$ | $\Sigma_0^{(1)}$ | $\Sigma_0^{(2)}$ | $\Sigma_0^{(3)}$ | $\Sigma_0^{(4)}$ |
| Post-processed posterior | 3.51 | 2.79 | 4.2 | 2.92 | 2.38 | 1.88 | 3.01 | 2.05 |
| Dual post-processed posterior | 6.40 | 3.97 | 7.67 | 5.67 | 5.84 | 3.64 | 7.02 | 5.23 |
| Banded sample covariance | 3.00 | 1.78 | 3.47 | 2.89 | 2.06 | 1.51 | 2.52 | 2.52 |
| Dual Maximum likelihood | 5.75 | 3.59 | 7.13 | 5.26 | 4.36 | 2.84 | 5.5 | 4.52 |

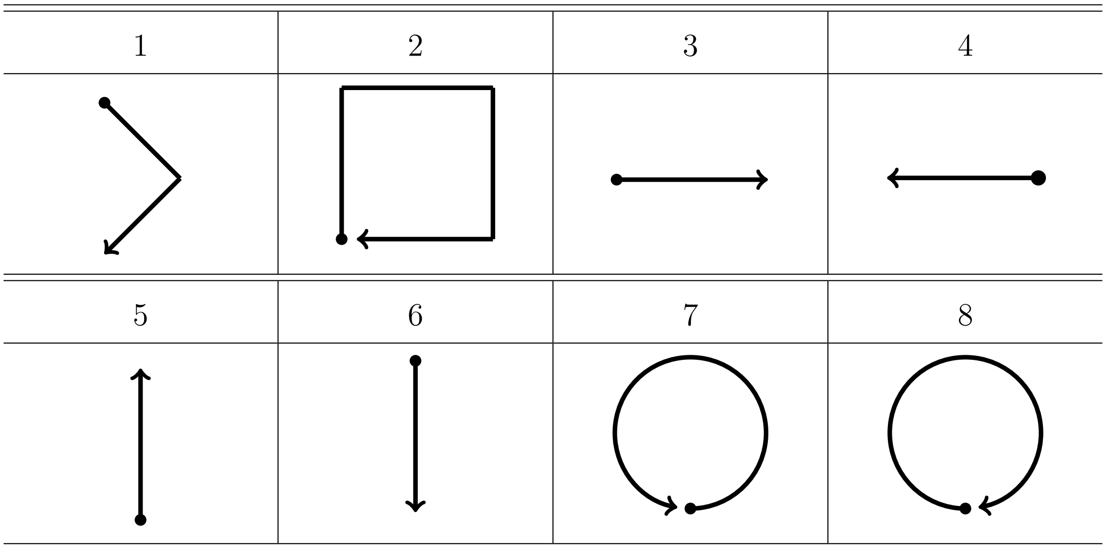


Table 2: Eight types of gestures. A dot and an arrow denote a starting point and an endpoint, respectively. This figure is adopted from Liu et al. (2009).

Each observation corresponds to one of the eight motions, which is described by accelerations in $x, y$ and $z$ axes at 315 time points. Thus, each observation is a 945-dimensional vector. Since there is a natural order among observations in time, we assume the covariance of observation has band structure. We apply the post-processed posterior to estimate the covariance matrix.

The predictive density of a new observation $z$ for the $j$th group is defined as

$$p_j^*(z \mid \mathbb{X}_n) = \iint p(z \mid \mu_j, \Sigma)\pi(\mu_j, \Sigma \mid \mathbb{X}_n) d\mu_j d\Sigma,$$

where $\mu_j$ is the $j$th group mean, $\Sigma$ is a covariance matrix, and $p(z \mid \mu_j, \Sigma)$ is the density of $N(z \mid \mu_j, \Sigma)$. To focus on inference for the covariance matrix, we fix $\mu_j = \hat{\mu}_j$ and consider an approximated predictive density for the $j$th group

$$p_j(z \mid \mathbb{X}_n) = \int p(z \mid \hat{\mu}_j, \Sigma)\pi(\Sigma \mid \mathbb{X}_n) d\Sigma,$$

where $\hat{\mu}_j = n_j^{-1} \sum_{x \in D_j} x$, $n_j = |D_j|$ and $D_j$ is a set of observations in the $j$th group. We use the Monte Carlo method for numerical integration. First, sample $\Sigma^{(t)}$ from the inverse-Wishart distribution

$$\Sigma^{(t)} \sim IW(A_0 + nS, \nu_0 + n), \quad t = 1, \ldots, m,$$

where $S = n^{-1} \sum_{i=1}^{g} n_i S_i$ , $n = \sum_{i=1}^{g} n_i$ and $S_i = n_i^{-1} \sum_{x \in D_i} (x - \hat{\mu_i})(x - \hat{\mu_i})^T$. In this experiment, the number of posterior samples $m$ is set to 1000. After that, we calculate

$$\hat{p}_j(z \mid \mathbb{X}_n) = \frac{1}{m} \sum_{t=1}^{m} p\{z \mid \hat{\mu}_j, f(\Sigma^{(t)})\},$$

where the post-processing function $f(\cdot)$ is chosen as $B_k^{(\epsilon)}(\cdot)$. To select the bandwidth $k$ and $\epsilon$, we use leave-one-out cross-validation as we did in the simulation.

We compared our method with linear discriminant analysis using the sample covariance, banding estimator. Since the sample covariance is not positive-definite, we add $\epsilon_n I_p$, where $\epsilon_n$ is chosen by leave-one-out cross-validation. For Bayesian methods, we classify $z$ to class $\hat{j} := \operatorname{argmax}_j \pi_j \hat{p}_j(z|\mathbb{X}_n)$. The performance is summarized in the accuracy column of Table 3.

Table 3: Performance of Linear discriminant analysis

| Method | Accuracy | Cross-entropy |
|---|---|---|
| Sample covariance | 75.32% | 1.318 |
| Inverse-Wishart posterior | 76.30% | 0.877 |
| Banding covariance | 86.54% | 0.881 |
| Post-processed posterior | 86.57% | 0.856 |

Estimators exploiting banded and bandable structure attains better performance. It implies the advantage of banded or bandable covariance matrices because the data has a time order. Moreover, Post-processed posterior methods show comparable performance to the frequentist alternatives. If we consider the estimated probability, not the estimated class, Bayesian methods give a more reliable estimator since it incorporates uncertainty of the covariance, which is pointed by Du and Ghosal (2018). To support the argument, we compare the methods with the cross-entropy loss, which is defined as

$$-\sum_{j=1}^{8} I(y=j) \log \hat{p}_j(z \mid \mathbb{X}_n),$$

for a test data $(y, z) \in \{1, \ldots, 8\} \times \mathbb{R}^{945}$. To make the cross-entropy loss stable, the estimated probabilities are adjusted so that the lowest estimated probability is larger than 0.1%. The average of the cross-entropy loss for the test set is in the cross-entropy column in Table 3. The post-processed posterior is the best in the all aspects, and it is notable that the cross-entropy loss by inverse-Wishart distribution is lower than that by banding covariance estimator.

# 4 proofs of theorems 1-3, S1-S3 and related lemmas

We define the sub-block transformation

$$\begin{aligned} M_l^{(k)}(\Sigma) &= (\sigma_{ij}^*)_{k\times k}, \\ \sigma_{ij}^* &= \sigma_{l-1+i,l-1+j} \\ \hat{\Sigma}_n &:= (nS_n + A_n)/(n+\nu_n - 2p + k - 1), \end{aligned}$$

and the tapering operation of matrices

$$T_k(\Sigma) = (w_{ij}^{(k)}\sigma_{ij}), \tag{2}$$

where $\Sigma = (\sigma_{ij}, 1 \le i, j \le p)$ and

$$w_{ij}^{(k)} = \begin{cases} 1, & \text{when } \mid i-j \mid \le k/2 \\ 2 - \dfrac{\mid i-j \mid}{k/2}, & \text{when } k/2 < \mid i-j \mid < k \\ 0, & \text{otherwise.} \end{cases}$$

**Lemma 4.1** *Suppose $\Sigma_0 = \Sigma_0(\theta_1, 0)$ is the true $k$-banded covariance matrix and the regularity conditions (3) hold. Then,*

$$n^{1/2}\begin{bmatrix} \{\hat{\theta}_1^* - \theta_1(\Sigma_0)\} \\ \{\hat{\theta}_1 - \theta_1(\Sigma_0)\} \end{bmatrix} \overset{d}{\longrightarrow} N\left(0, \begin{bmatrix} \mathcal{I}_{11\cdot 2}^{-1}\{\theta_1(\Sigma_0), 0\} & \mathcal{I}_{11}^{-1}\{\theta_1(\Sigma_0), 0\} \\ \mathcal{I}_{11}^{-1}\{\theta_1(\Sigma_0), 0\} & \mathcal{I}_{11}^{-1}\{\theta_1(\Sigma_0), 0\} \end{bmatrix}\right)$$

*as $n \to \infty$.*

**Proof** By Taylor's theorem,

$$\begin{aligned} \sqrt{n}\{\hat{\theta}_1^* - \theta_1(\Sigma_0)\} &= -[L_n''\{\theta_1(\Sigma_0), 0\}^{-1}]_{11}[L_n'\{\theta_1(\Sigma_0), 0\}]_1 - [L_n''\{\theta_1(\Sigma_0), 0\}^{-1}]_{12}[L_n'\{\theta_1(\Sigma_0), 0\}]_2 \\ \sqrt{n}\{\hat{\theta}_1 - \theta_1(\Sigma_0)\} &= -[L_n''\{\theta_1(\Sigma_0), 0\}]_{11}^{-1}[L_n'\{\theta_1(\Sigma_0), 0\}]_1, \end{aligned}$$

which are expressed in the matrix form

$$\sqrt{n}\begin{bmatrix} (\hat{\theta}_1^* - \theta_1(\Sigma_0)) \\ (\hat{\theta}_1 - \theta_1(\Sigma_0)) \end{bmatrix} = \begin{bmatrix} -[L_n''\{\theta_1(\Sigma_0), 0\}^{-1}]_{11} & -[L_n''\{\theta_1(\Sigma_0), 0\}^{-1}]_{12} \\ -[L_n''\{\theta_1(\Sigma_0), 0\}]_{11}^{-1} & 0 \end{bmatrix}\begin{bmatrix} [L_n'(\theta_{01}, 0)]_1 \\ [L_n'(\theta_{01}, 0)]_2 \end{bmatrix}.$$

Since

$$\sqrt{n}L_n'(\theta_{01},0) \xrightarrow{d} N(0,\mathcal{I}(\theta_{01},0)),$$

$$\begin{aligned}
\sqrt{n}\begin{bmatrix}(\hat{\theta}_1^* - \theta_{01})\\ (\hat{\theta}_1 - \theta_{01})\end{bmatrix} &\xrightarrow{d} \begin{bmatrix}(\mathcal{I}(\theta_{01},0)^{-1})_{11} & (\mathcal{I}(\theta_{01},0)^{-1})_{12}\\ (\mathcal{I}(\theta_{01},0))_{11}^{-1} & 0\end{bmatrix} N(0,\mathcal{I}_0)\\
&= N\left(0, \begin{bmatrix}[\mathcal{I}_{11\cdot 2}\{\theta_1(\Sigma_0),0\}]^{-1} & [\mathcal{I}_{11}\{\theta_1(\Sigma_0),0\}]^{-1}\\ [\mathcal{I}_{11}\{\theta_1(\Sigma_0),0\}]^{-1} & [\mathcal{I}_{11}\{\theta_1(\Sigma_0),0\}]^{-1}\end{bmatrix}\right).
\end{aligned}$$

**Lemma 4.2** *Let $\Omega_n \sim W_p(\nu_n, \nu_n^{-1}I_p)$ with $c\nu_n \geq p$ for some constant $0 < c < 1$. Then ,*

$$\begin{aligned}
pr\{\lambda_{max}(\Omega_n) \geq c_1\} &\leq 2e^{-\nu_n/2},\\
pr\{\lambda_{min}(\Omega_n) \leq c_2\} &\leq 2e^{-\nu_n\{1-(p/\nu_n)^{1/2}\}^2/8}
\end{aligned}$$

*for any constant $c_1 \geq \{2 + (p/\nu_n)^{1/2}\}^2$ and $0 < c_2 \leq \{1 - (p/\nu_n)^{1/2}\}^2/4$.*

**Proof** See p. 87 of Lee (2018) or Lemma B.7 in the supplementary material of Lee and Lee (2018).

**Lemma 4.3** *When $X \sim gamma(\gamma/2, \gamma/2)$ and $x \geq 0$, it satisfies*

$$pr(|X-1| \geq x) \leq \begin{cases} 2\exp(-\gamma x^2/8) & \text{for } 0 \leq x \leq 1,\\ 2\exp(-\gamma x/8) & \text{for } x > 1\end{cases}$$

**Proof** For $|\lambda| < \gamma/4$,

$$E(e^{\lambda(X-1)}) \leq e^{\frac{2\lambda^2}{\gamma}}.$$

Because for $|\lambda| < \gamma/4$,

$$\begin{aligned}
\log\left\{E(e^{\lambda(X-1)})\right\} &= -\lambda - \gamma\log(1-2\lambda/\gamma)/2\\
&\leq -\lambda - \gamma\{-2\lambda/\gamma - (2\lambda/\gamma)^2\}/2\\
&= 2\lambda^2/\gamma.
\end{aligned}$$

The second inequality is satisfied since $\log(1-x) \geq -x - x^2$ for all $|x| < 1/2$. Thus, $E(e^{\lambda(X-1)}) \leq \exp(2\lambda^2/\gamma)$ and this is the sub-exponontial distribution with $(2/(\gamma)^{1/2}, 4/\gamma)$. Using the Bernstein inequality of the sub-exponential tail bound (Proposition 2.9 in Wainwright (2019)), we get

$$pr(|X-1| \geq x) \leq \begin{cases} 2\exp(-\gamma x^2/8) & \text{for } 0 \leq x \leq 1, \\ 2\exp(-\gamma x/8) & \text{for } x > 1 \end{cases}$$

**Lemma 4.4** *If* $\Omega_n \sim W_k(\gamma, \gamma^{-1} I_k)$ *and* $x \geq 0$,

$$pr(||\Omega_n - I_k|| \geq x) \leq \begin{cases} 2\{5^k \exp(-\gamma x^2/2^7)\} & \textit{for } 0 \leq x \leq 1 \\ 2\{5^k \exp(-\gamma x/2^7)\} & \textit{for } x > 1. \end{cases}$$

**Proof** For any $k \times k$ matrix $A$, there exists a set of vectors $v_j \in \mathbb{R}^k$ for $j = 1, \ldots, 5^k$ with $||v_j||_2 = 1$ such that $||A|| \leq 4 \sup_{j \leq 5^k} |v_j^T A v_j|$ (Cai and Zhou; 2010).

Since $\Omega_n \sim W_k(\gamma, \gamma^{-1} I_k)$ and $v^T \Omega_n v \sim gamma(\gamma/2, \gamma/2)$ for all vector $v \in \mathbb{R}^p$ with $||v||_2 = 1$, by Lemma 4.3,

$$\begin{aligned} pr(||\Omega_n - I_k|| \geq x) &\leq pr(4 \sup_{j \leq 5^k} |v_j^T \Omega_n v_j - 1| \geq x) \\ &\leq 5^k \sup_{j \leq 5^k} pr(|v_j^T \Omega_n v_j - 1| \geq x/4), \\ &\leq \begin{cases} 2\{5^k \exp(-\gamma x^2/2^7)\} & \text{for } 0 \leq x \leq 1 \\ 2\{5^k \exp(-\gamma x/2^7)\} & \text{for } x > 1. \end{cases} \end{aligned}$$

**Lemma 4.5** *Let* $\tau_2 := ||M_l^{(k)}(\Sigma_0)||$. *Then, for* $x \geq \tau_2\{2 + (k/n)^{1/2}\}^2 + (||A_n||)/(n + \nu_n - 2p + k - 1)$,

$$pr_{\Sigma_0}\Big(||M_l^{(k)}(\hat{\Sigma}_n)|| > x\Big) < 2\exp(-n/2).$$

**Proof**

$$\begin{aligned}
pr_{\Sigma_0}\Big(||M_l^{(k)}(\hat{\Sigma}_n)|| > x\Big) &\leq pr_{\Sigma_0}\Big(||M_l^{(k)}(S_n)|| + \frac{||A_n||}{n+\nu_n-2p+k-1} > x\Big) \\
&\leq pr\Big(||M_l^{(k)}(\Sigma_0)^{1/2}||\ ||\Omega_n||\ ||M_l^{(k)}(\Sigma_0)^{1/2}|| > x - \frac{||A_n||}{n+\nu_n-2p+k-1}\Big) \\
&\leq pr\Bigg\{||\Omega_n|| > \tau_2^{-1}\Big(x - \frac{||A_n||}{n+\nu_n-2p+k-1}\Big)\Bigg\}, \qquad (3)
\end{aligned}$$

where $\Omega_n \sim W_k(n, n^{-1}I_k)$. Since $x \geq \tau_2\{2+(k/n)^{1/2}\}^2 + ||A_n||/(n+\nu_n-2p+k-1)$, we have

$$pr_{\Sigma_0}\Big(||M_l^{(k)}(\hat{\Sigma}_n)|| > x\Big) \leq pr\Big[\{\lambda_{\max}(\Omega_n)\}^{1/2} > \{2+(k/n)^{1/2}\}\Big].$$

Corollary 5.35 in Eldar and Kutyniok (2012) says

$$pr\Big\{\lambda_{\max}(\Omega_n)^{1/2} \geq 1 + (k/n)^{1/2} + t/(n)^{1/2}\Big\} \leq 2e^{-t^2/2}.$$

Setting $t = n^{1/2}$ in the above inequality, we have

$$pr_{\Sigma_0}\Big(||M_l^{(k)}(\hat{\Sigma}_n)|| > x\Big) \leq 2e^{-n/2}.$$

**Lemma 4.6** *Let* $\tau_2 := ||M_l^{(k)}(\Sigma_0)||$. *Then, for* $x \geq (\max[||A_n||/\{2(n+\nu_n-2p+k-1)\}, \tau_2/2\{1+k/n+2(k/n)^{1/2}\}])^{1/2}$,

$$E_{\Sigma_0}(||\ M_l^{(k)}(\hat{\Sigma}_n)\ ||^2\ I(||\ M_l^{(k)}(\hat{\Sigma}_n)\ || > x)) < \Big\{\frac{64\tau_2}{n} + \Big(\frac{64\tau_2}{n}\Big)^2\Big\}e^{-nx^{1/2}/(16\tau_2)}.$$

**Proof** Using the change of variable formula and (3), we have

$$\begin{aligned}
E_{\Sigma_0}\{||M_l^{(k)}(\hat{\Sigma}_n)||^2 I(||M_l^{(k)}(\hat{\Sigma}_n)|| > x)\} &\leq 2\int_{x^{1/2}}^{\infty} u pr_{\Sigma_0}(||M_l^{(k)}(\hat{\Sigma}_n)|| \geq u)du \\
&\leq 2\int_{x^{1/2}}^{\infty} u pr\Bigg\{||\Omega_n|| \geq \tau_2^{-1}\Big(u - \frac{||A_n||}{n+\nu_n-2p+k-1}\Big)\Bigg\},
\end{aligned}$$

where $\Omega_n \sim W_k(n, n^{-1}I_k)$. Setting $t = n^{1/2}([\tau_2^{-1}\{u - ||\ A_n\ ||\ /(n+\nu_n-2p+k-1)\}]^{1/2} - 1 - (k/n)^{1/2})$ in Corollary 5.35 in Eldar and Kutyniok (2012), we get

$$pr\Bigg\{||\Omega_n|| \geq \tau_2^{-1}\Big(u - \frac{||A_n||}{n+\nu_n-p+k}\Big)\Bigg\} \leq 2e^{-n([\tau_2^{-1}\{u-||A_n||/(n+\nu_n-p+k)\}]^{1/2}-1-(k/n)^{1/2})^2/2}.$$

Applying the above inequality, we have, for $x^2 \geq \max[||A_n||/\{2(n+\nu_n-2p+k-1)\}, \tau_2/2\{1+k/n+2(k/n)^{1/2}\}]$,

$$\begin{aligned} E_{\Sigma_0}\{||M_l^{(k)}(\hat{\Sigma}_n)||^2 I(||M_l^{(k)}(\hat{\Sigma}_n)||>x)\} &\leq 4\int_{x^{1/2}}^{\infty} u e^{-n([\tau_2^{-1}\{u-||A_n||/(n+\nu_n-2p+k-1)\}]^{1/2}-1-(k/n)^{1/2})^2/2} du \\ &\leq 4\int_{x^{1/2}}^{\infty} u e^{-nu/(16\tau_2)} du \\ &\leq \Big\{\frac{64\tau_2}{n}+\Big(\frac{64\tau_2}{n}\Big)^2\Big\} e^{-nx^{1/2}/(16\tau_2)}. \end{aligned}$$

**Lemma 4.7** *Let* $\tau_1 := \lambda_{\min}\{M_l^{(k)}(\Sigma_0)\}$. *If* $x > 4\tau_1^{-1}\{1+(\nu_n-2p+k-1)/n\}/\{1-(k/n)^{1/2}\}^2$, *then*

$$pr_{\Sigma_0}\Big(||M_l^{(k)}(\hat{\Sigma}_n)^{-1}||>x\Big) \leq 2\exp[-n\{1-(k/n)^{1/2}\}^2/8].$$

**Proof** It satisfies that

$$\begin{aligned} pr_{\Sigma_0}\Big(||M_l^{(k)}(\hat{\Sigma}_n)^{-1}||>x\Big) &\leq pr_{\Sigma_0}\Big(\frac{n+\nu_n-2p+k-1}{n}||M_l^{(k)}(S_n)^{-1}||>x\Big) \\ &\leq pr\Big(||M_l^{(k)}(\Sigma_0)^{-1/2}||\ ||\Omega_n^{-1}||\ ||M_l^{(k)}(\Sigma_0)^{-1/2}|| > \frac{n}{n+\nu_n-2p+k-1}x\Big) \\ &\leq pr\Big(||\Omega_n^{-1}|| > \tau_1\frac{n}{n+\nu_n-2p+k-1}x\Big) \\ &\leq pr\Big(\lambda_{\min}(\Omega_n) < \tau_1^{-1}\frac{n+\nu_n-2p+k-1}{n}x^{-1}\Big), \end{aligned}$$

where $\Omega_n \sim W_k(n, n^{-1}I)$. Since $x > 4\tau_1^{-1}\{1+(\nu_n-2p+k-1)/n\}/\{1-(k/n)^{1/2}\}^2$, by Lemma 4.2, we have

$$pr_{\Sigma_0}\Big(||M_l^{(k)}(\hat{\Sigma}_n)^{-1}||>x\Big) \leq pr\Big[\lambda_{\min}(\Omega_n) < \{1-(k/n)^{1/2}\}^2/4\Big] \leq 2e^{[-n\{1-(k/n)^{1/2}\}^2/8]}.$$

**Lemma 4.8** *Let* $\tau_1 := \lambda_{\min}\{M_l^{(k)}(\Sigma_0)\}$, $\tau_2 := ||M_l^{(k)}(\Sigma_0)||$, $z = 4\tau_2(1+k/n+2(k/n)^{1/2})$, $C = 8||A_n||^4/(n+\nu-2p+k-1)^4 + z^4/4$ *and* $C_1 = C + 64(8\tau_2 z^3/n + 3(8\tau_2)^2 z^2/n^2 + 6z(8\tau_2)^3/n^3 + 6(8\tau_2)^4/n^4)\exp\{-nz/(8\tau_2)\}$. *If* $x > 4\tau_1^{-1}\{1+(\nu_n-2p+k-1)/n\}/\{1-(k/n)^{1/2}\}^2$, *then*

$$E_{\Sigma_0}\{||M_l^{(k)}(\hat{\Sigma}_n)||^2 I(||M_l^{(k)}(\hat{\Sigma}_n)^{-1}||>x)\} < (2C_1)^{1/2}\exp\{-n(1-(k/n)^{1/2})^2/16\}.$$

**Proof** We have

$$
\begin{aligned}
E_{\Sigma_0}(||M_l^{(k)}(\hat{\Sigma}_n)||^4) &\leq 8\frac{||A_n||^4}{(n+\nu-2p+k-1)^4} + 8E_{\Sigma_0}(||M_l^{(k)}(S_n)||^4) \\
&\leq C + 32\int_z^\infty u^3 pr_{\Sigma_0}(||M_l^{(k)}(S_n)|| > u)du \\
&\leq C + 32\int_z^\infty u^3 pr(||\Omega_n|| > \tau_2^{-1}u)du \\
&\leq C + 64\int_z^\infty u^3 \exp[-n\{(\tau_2^{-1}u)^{1/2} - 1 - (k/n)^{1/2}\}^2/2]du \\
&\leq C + 64\int_z^\infty u^3 \exp\{-nu/(8\tau_2)\}du \\
&\leq C + 64(8\tau_2 z^3/n + 3(8\tau_2)^2 z^2/n^2 + 6z(8\tau_2)^3/n^3 + 6(8\tau_2)^4/n^4)\exp\{-nz/(8\tau_2)\},
\end{aligned}
$$

where $\tau_2 = ||M_l^{(k)}(\Sigma_0)||$, $\Omega_n \sim W_k(n, n^{-1}I_k)$, $z = 4\tau_2(1 + k/n + 2(k/n)^{1/2})$ and $C = 8||A_n||^4/(n+\nu-2p+k-1)^4 + z^4/4$. The fourth inequality can be obtained by applying Corollary 5.35 in Eldar and Kutyniok (2012) with $t = (n)^{1/2}\{(\tau_2^{-1}u)^{1/2} - 1 - (k/n)^{1/2}\}$. Thus, by Lemma 4.7, for $x > 4\tau_1^{-1}\{1 + (\nu_n - 2p + k - 1)/n\}/\{1 - (k/n)^{1/2}\}^2$,

$$
\begin{aligned}
E_{\Sigma_0}\{||M_l^{(k)}(\hat{\Sigma}_n)||^2 I(||M_l^{(k)}(\hat{\Sigma}_n)^{-1}|| > x)\} &\leq \left\{E_{\Sigma_0}(||M_l^{(k)}(\hat{\Sigma}_n)||^4) pr_{\Sigma_0}(||M_l^{(k)}(\hat{\Sigma}_n)^{-1}|| > x)\right\}^{1/2} \\
&\leq \left[E_{\Sigma_0}(||M_l^{(k)}(\hat{\Sigma}_n)||^4) 2\exp\{-n(1-(k/n)^{1/2})^2/8\}\right]^{1/2} \\
&\leq (2C_1)^{1/2}\exp\{-n(1-(k/n)^{1/2})^2/16\},
\end{aligned}
$$

where $C_1 = C + 64(8\tau_2 z^3/n + 3(8\tau_2)^2 z^2/n^2 + 6z(8\tau_2)^3/n^3 + 6(8\tau_2)^4/n^4)\exp\{-nz/(8\tau_2)\}$.

**Lemma 4.9** *Let $\Sigma = (\sigma_{ij})_{p\times p} \sim IW_p(A, \nu)$ and $A = (a_{ij})_{p\times p}$. Then,*

$$
E(\sigma_{jj}^r) = a_{ii}^r \frac{1}{2^r}\frac{\Gamma(\frac{\nu-2p}{2} - r)}{\Gamma(\frac{\nu-2p}{2})}, \quad \frac{\nu-2p}{2} > r > 0, j = 1.2, \ldots, p.
$$

*Furthermore, if $r$ is a natural number, the RHS simplifies to $(a_{ii}^r)/\{\prod_{v=1}^{r}(\nu - 2p - 2v)\}$.*

**of Lemma 4.9** Since $\sigma_{jj} \sim IW_1(a_{ii}, \nu - 2p + 2)$ for any $j = 1, 2, \ldots, p$ (Press (2005)), we have $\sigma_{jj}^{-1} \sim W_1(\nu - 2p, a_{ii}^{-1}) \stackrel{d}{=} a_{ii}^{-1}\chi^2_{\nu-2p}$. Using the fact that $E(X^{-r}) = [\Gamma\{(\nu-2p)/2 - r\}]/[2^r\Gamma\{(\nu-2p)/2\}]$ for $X \sim \chi^2_{\nu-2p}$, we complete the proof.

**Lemma 4.10** *Suppose $X_1, \dots, X_n$ are independent and identically distributed sample from $N_p(0, \Sigma_0)$ and the prior distribution of $\Sigma$, $\pi^i$, is $IW_p(A_n, \nu_n)$ with $||A_n|| = o(n)$ and $(\nu_n - 2p) = o(n)$. Then*

$$E_{\Sigma_0}\{E^{\pi^i}(\max_{1\le l\le p-k+1} ||M_l^{(k)}(\Sigma - \hat{\Sigma})||^2 \mid \mathbb{X}_n)\} \le C\frac{k+\log p}{n} + o\Big(\frac{k+\log p}{n}\Big),$$

*where $C = 2^{10}\log 5\{(2||\Sigma_0||)^{1/2} \vee 8||\Sigma_0||\}^3/||\Sigma_0^{-1}||$.*

**Proof** The expectation term can be decomposed as

$$\begin{aligned}
& E_{\Sigma_0}\{E^{\pi^i}(\max_{1\le l\le p-k+1} ||M_l^{(k)}(\Sigma - \hat{\Sigma})||^2 \mid \mathbb{X}_n)\} \\
= \;& E_{\Sigma_0}\Big\{E^{\pi^i}(\max_{1\le l\le p-k+1} ||M_l^{(k)}(\Sigma - \hat{\Sigma})||^2 \mid \mathbb{X}_n) \\
\times \;& I(\max_{1\le l\le p-k+1} ||M_l^{(k)}(\hat{\Sigma})|| \le C_1, \max_{1\le l\le p-k+1} ||M_l^{(k)}(\hat{\Sigma})^{-1}|| \le C_2)\Big\} \qquad (4) \\
+ \;& E_{\Sigma_0}\Big\{E^{\pi^i}(\max_{1\le l\le p-k+1} ||M_l^{(k)}(\Sigma - \hat{\Sigma})||^2 \mid \mathbb{X}_n) \\
\times \;& I(\max_{1\le l\le p-k+1} ||M_l^{(k)}(\hat{\Sigma})|| > C_1 \text{ or } \max_{1\le l\le p-k+1} ||M_l^{(k)}(\hat{\Sigma})^{-1}|| > C_2)\Big\} \qquad (5)
\end{aligned}$$

for any positive constants $C_1$ and $C_2$. Let

$$\begin{aligned}
I(U_1) &:= I(\max_{1\le l\le p-k+1} ||M_l^{(k)}(\hat{\Sigma})|| \le C_1, \max_{1\le l\le p-k+1} ||M_l^{(k)}(\hat{\Sigma})^{-1}|| \le C_2) \\
I(U_2) &:= I(\max_{1\le l\le p-k+1} ||M_l^{(k)}(\hat{\Sigma})|| > C_1 \text{ or } \max_{1\le l\le p-k+1} ||M_l^{(k)}(\hat{\Sigma})^{-1}|| > C_2)
\end{aligned}$$

The upper bound of (4) is given by

$$
\begin{aligned}
& E_{\Sigma_0}\{E^{\pi^i}(\max_{1\le l\le p-k+1}||M_l^{(k)}(\Sigma)||^2||M_l^{(k)}(\Sigma)^{-1}M_l^{(k)}(\hat\Sigma)-I||^2\mid \mathbb{X}_n)I(U_1)\}\\
\le\ & E_{\Sigma_0}\{E^{\pi^i}(\max_{1\le l\le p-k+1}||M_l^{(k)}(\Sigma)||^2||M_l^{(k)}(\hat\Sigma)||\ ||M_l^{(k)}(\hat\Sigma)^{-1}||\ ||\Omega_{n,l}^{(k)}-I||^2\mid \mathbb{X}_n)I(U_1)\}\\
\le\ & C_1C_2C_3^2E_{\Sigma_0}\{E^{\pi^i}(\max_{1\le l\le p-k+1}||\Omega_{n,l}^{(k)}-I||^2\mid \mathbb{X}_n)I(U_1)\}\\
+\ & C_1C_2E_{\Sigma_0}\{E^{\pi^i}(\max_{1\le l\le p-k+1}||M_l^{(k)}(\Sigma)||^2\ ||\Omega_{n,l}^{(k)}-I||^2 I(\max_{1\le l\le p-k+1}||M_l^{(k)}(\Sigma)||>C_3)\mid \mathbb{X}_n)I(U_1)\}\\
\le\ & C_1C_2C_3^2E_{\Sigma_0}\Big\{\int_0^\infty pr^{\pi_n}(\max_{1\le l\le p-k+1}||\Omega_{n,l}^{(k)}-I||^2>u\mid \mathbb{X}_n)duI(U_1)\Big\}\\
+\ & C_1C_2E_{\Sigma_0}[\{E^{\pi^i}(\max_{1\le l\le p-k+1}||\Omega_{n,l}^{(k)}-I||^4 I(\max_{1\le l\le p-k+1}||M_l^{(k)}(\Sigma)||>C_3)\mid \mathbb{X}_n)\}^{1/2}\\
\times\ & \{E^{\pi^i}(\max_{1\le l\le p-k+1}||M_l^{(k)}(\Sigma)||^4\mid \mathbb{X}_n)\}^{1/2}I(U_1)]\\
\le\ & C_1C_2C_3^2\Big\{x^2+\sum_{l=1}^{p-k+1}E_{\Sigma_0}\int_{x^2}^\infty pr^{\pi^i}(||\Omega_{n,l}^{(k)}-I||^2>u\mid \mathbb{X}_n)du\Big\}\\
+\ & C_1C_2E_{\Sigma_0}\Big[\{E^{\pi^i}(\max_{1\le l\le p-k+1}||\Omega_{n,l}^{(k)}-I||^8\mid \mathbb{X}_n)\}^{1/4}\times\{E^{\pi^i}(\max_{1\le l\le p-k+1}||M_l^{(k)}(\Sigma)||^4\mid \mathbb{X}_n)\}^{1/2}\\
\times\ & \{pr^{\pi^i}(\max_{1\le l\le p-k+1}||M_l^{(k)}(\Sigma)||>C_3\mid \mathbb{X}_n)\}^{1/4}I(U_1)\Big]
\end{aligned}
$$

for any positive constant $C_3>0$ and any $x>0$. Here $\Omega_{n,l}^{(k)}:=M_l^{(k)}(\hat\Sigma)^{1/2}M_l^{(k)}(\Sigma)^{-1}M_l^{(k)}(\hat\Sigma)^{1/2}$ and it satisfies that

$$\Omega_{n,l}^{(k)}\sim W_k\Big(n+\nu_n-2p+k-1,\frac{1}{n+\nu_n-2p+k-1}I_k\Big).$$

By Lemma 4.4,

$$
\begin{aligned}
& \int_{x^2}^\infty pr^{\pi^i}(||\Omega_{n,l}^{(k)}-I||^2>u\mid \mathbb{X}_n)du\\
\le\ & 2\int_{x^2}^\infty u\{pr^{\pi^i}(||\Omega_{n,l}^{(k)}-I||>u\mid \mathbb{X}_n)\}du\\
\le\ & 2\int_{x^2}^1 u\{pr^{\pi^i}(||\Omega_{n,l}^{(k)}-I||>u\mid \mathbb{X}_n)\}du+2\int_1^\infty u\{pr^{\pi^i}(||\Omega_{n,l}^{(k)}-I||>u\mid \mathbb{X}_n)\}du\\
\le\ & 4(5^k)\int_{x^2}^\infty u\exp(-nu^2/2^7)du+4(5^k)\int_1^\infty u\exp(-nu/2^7)du\\
\le\ & 2^8(5^k)\exp(-nx^2/2^7)/n+(2^95^k/n+2^{16}5^k/n^2)\exp(-n/2^7)
\end{aligned}
$$

Using this inequality, we obtain

$$\begin{aligned} & \sum_{l=1}^{p-k+1} E_{\Sigma_0}\Big\{\int_{x^2}^{\infty} pr^{\pi^i}\Big(||\Omega_{n,l}^{(k)} - I||^2 > u \mid \mathbb{X}_n\Big) du\Big\} \\ \leq \;& p5^k\{2^8 \exp(-nx^2/2^7)/n + (2^9/n + 2^{16}/n^2)\exp(-n/2^7)\}. \end{aligned}$$

By similar arguments,

$$\begin{aligned} & \{E^{\pi^i}(\max_{1\leq l\leq p-k+1} ||\Omega_{n,l}^{(k)} - I||^8 \mid \mathbb{X}_n)\}^{1/4} \\ \leq \;& [1 + \sum_{l=1}^{p-k+1} E_{\Sigma_0}\{\int_1^{\infty} pr^{\pi^i}(||\Omega_{n,l}^{(k)} - I||^8 > u \mid \mathbb{X}_n) du\}]^{1/4} \\ \leq \;& 1 + \Big[8 \sum_{l=1}^{p-k+1} E_{\Sigma_0}\{\int_1^{\infty} u^7 pr^{\pi^i}(||\Omega_{n,l}^{(k)} - I|| > u \mid \mathbb{X}_n) du\}\Big]^{1/4} \\ \leq \;& 1 + \Big[2^4 5^k \sum_{l=1}^{p-k+1} E_{\Sigma_0}\Big\{\int_1^{\infty} u^7 \exp(-nu/2^7) du\Big\}\Big]^{1/4} \\ \leq \;& 1 + (5^{k/4}) p^{1/4} \frac{2^{11/4}}{n^{1/4}} \Big\{\sum_{i=0}^{7} \frac{7!}{(7-i)!}\Big(\frac{2^7}{n}\Big)^i\Big\}^{1/4}. \end{aligned}$$

Also if $C_1 C_3^{-1} \leq [1 - \{k/(n+k)\}^{1/2}]^2/4$, it satisfies that

$$\begin{aligned} & pr^{\pi^i}\{(\min_{1\leq l\leq p-k+1} ||M_l^{(k)}(\Sigma)|| > C_3) \mid \mathbb{X}_n\} I(U_1) \\ \leq \;& pr^{\pi^i}[\{\min_{1\leq l\leq p-k+1} \lambda_{\min}(M_l^{(k)}(\Sigma)^{-1}) < C_3^{-1}\} \mid \mathbb{X}_n] I(U_1) \\ \leq \;& pr^{\pi^i}[\{\min_{1\leq l\leq p-k+1} \lambda_{\min}(\Omega_{n,l}^{(k)})/||M_l^{(k)}(\hat{\Sigma})|| < C_3^{-1}\} \mid \mathbb{X}_n] I(U_1) \\ \leq \;& pr^{\pi^i}[\{\min_{1\leq l\leq p-k+1} \lambda_{\min}(\Omega_{n,l}^{(k)}) < C_1 C_3^{-1}\} \mid \mathbb{X}_n] I(U_1) \\ \leq \;& 2p \exp[-(\nu_n^*)\{1 - (k/\nu_n^*)^{1/2}\}^2/8] \\ \leq \;& 2p \exp(-(n+k)[1 - \{k/(n+k)\}^{1/2}]^2/8), \end{aligned}$$

where $\nu_n^* = n + \nu_n - 2p + k - 1$. The fourth inequality is satisfied by Lemma 4.2. Furthermore,

it can be easily shown that

$$
\begin{aligned}
E^{\pi^i}(\max_{1\le l\le p-k+1} ||M_l^{(k)}(\Sigma)||^4 \mid \mathbb{X}_n)I(U_1) &\le E^{\pi^i}[\max_{1\le l\le p-k+1} tr\{M_l^{(k)}(\Sigma)\}^4 \mid \mathbb{X}_n]I(U_1) \\
&\le k^4 E^{\pi^i}[\max_{1\le l\le p-k+1} \sum_{j=1}^{k}\{M_l^{(k)}(\Sigma)_{jj}\}^4 \mid \mathbb{X}_n]I(U_1) \\
&\le k^4 E^{\pi^i}\{\sum_{j=1}^{p}(\Sigma)_{jj}^4 \mid \mathbb{X}_n\}I(U_1) \\
&\le k^4 \sum_{j=1}^{p} \frac{\{(A_n)_{jj}+n(S_n)_{jj}\}^4}{(n+\nu_n-2p-8)^4} I(U_1) \\
&\le pk^4 \frac{(n+\nu_n-2p+k-1)^4}{(n+\nu_n-2p-8)^4} \max_{1\le l\le p-k+1} ||M_l^k(\hat{\Sigma})||^4 I(U_1) \\
&\le C_1^4 k^4 p \Big(\frac{n+\nu_n-2p+k-1}{n-8}\Big)^4.
\end{aligned}
$$

Then, (4) is bounded above by

$$
\begin{aligned}
& u_1(n,p,k,\nu_n,C_1,C_2) \\
:= \;& C_1C_2C_3^2\Big[x^2 + p5^k\{2^8\exp(-nx^2/2^7)/n + (2^9/n + 2^{16}/n^2)\exp(-n/2^7)\}\Big] \\
+ \;& \Big[C_1^3C_2 2^{1/4}k^2p^{3/4} + C_1^3C_2pk^2 2^3(5^{k/4})/n^{1/4}\Big\{\sum_{i=0}^{7}\frac{7!}{(7-i)!}\Big(\frac{2^7}{n}\Big)^i\Big\}^{1/4}\Big] \\
& \times \exp(-(n+k)[1-\{k/(n+k)\}^{1/2}]^2/32)\Big(\frac{n+\nu_n-2p+k-1}{n-8}\Big)^2,
\end{aligned}
$$

where we let $x^2 = 2^8\log 5(\log p + k)/n$ and $C_3 = 4C_1/[1-\{k/(n+k)\}^{1/2}]^2$.

On the other hand, (5) is bounded above by

$$
\begin{aligned}
& 2E_{\Sigma_0}\{E^{\pi^i}(\max_{1\le l\le p-k+1}||M_l^{(k)}(\Sigma)||^2 \mid \mathbb{X}_n)I(U_2)\} + 2E_{\Sigma_0}\{\max_{1\le l\le p-k+1}||M_l^{(k)}(\hat\Sigma)||^2 I(U_2)\} \\
\le\ & 2kE_{\Sigma_0}\Big(E^{\pi^i}[\sum_{j=1}^{p}\{(\Sigma)_{jj}\}^2|\mathbb{X}_n]I(U_2)\Big) + 2E_{\Sigma_0}\{\max_{1\le l\le p-k+1}||M_l^{(k)}(\hat\Sigma)||^2 I(U_2)\} \\
\le\ & \frac{2kp(n+\nu_n-2p+k-1)^2}{(n+\nu_n-2p-4)^2}E_{\Sigma_0}\Big\{\sum_{l=1}^{p-k+1}||M_l^{(k)}(\hat\Sigma_n)||^2 I(U_2)\Big\} + 2E_{\Sigma_0}\Big\{\max_{1\le l\le p-k+1}||M_l^{(k)}(\hat\Sigma)||^2 I(U_2)\Big\} \\
\le\ & (8kp+2)\sum_{l=1}^{p-k+1} E_{\Sigma_0}\{||M_l^{(k)}(\hat\Sigma)||^2 I(U_2)\} \\
\le\ & (8kp+2)\sum_{l=1}^{p-k+1}[E_{\Sigma_0}\{||M_l^{(k)}(\hat\Sigma)||^2 I(||M_l^{(k)}(\hat\Sigma)|| > C_1)\} + C_1^2\sum_{j=1}^{p-k+1} pr_{\Sigma_0}(||M_j^{(k)}(\hat\Sigma)|| > C_1)] \\
+\ & (8kp+2)\sum_{l=1}^{p-k+1}\Big[E_{\Sigma_0}\{||M_l^{(k)}(\hat\Sigma)||^2 I(||M_l^{(k)}(\hat\Sigma)^{-1}|| > C_2)\} + C_1^2\sum_{j=1}^{p-k+1} pr_{\Sigma_0}(||M_j^{(k)}(\hat\Sigma)^{-1}|| > C_2)\Big].
\end{aligned}
$$

The first inequality is obtained since

$$
\begin{aligned}
\max_{1\le l\le p-k+1}||M_l^{(k)}(\Sigma)||^2 &\le \max_{1\le l\le p-k+1} tr\{M_l^{(k)}(\Sigma)\}^2 \\
&\le k\sum_{j=1}^{p}\{(\Sigma)_{jj}\}^2.
\end{aligned}
$$

Applying Lemmas 4.6, 4.8 by setting

$$
\begin{aligned}
C_1 &= \max\Big\{\Big(\max\Big[\frac{||A_n||}{2n}, \frac{\tau_2\{1+k/n+2(k/n)^{1/2}\}}{2}\Big]\Big)^{1/2}, \tau_2\{2+(k/n)^{1/2}\}^2 + \frac{||A_n||}{n}\Big\}, \\
C_2 &= 4\tau_1^{-1}\{1+(\nu_n-2p+k-1)/n\}/\{1-(k/n)^{1/2}\}^2,
\end{aligned}
$$

we obtain an upper bound of (5) as

$$
\begin{aligned}
& u_2(n,p,k,||A_n||,\lambda_{\max}(\Sigma_0),\lambda_{min}(\Sigma_0),\nu) \\
:=\ & (8kp+2)p\Big\{\frac{64\tau_2}{n} + \Big(\frac{64\tau_2}{n}\Big)^2\Big\}e^{-nC_1^{1/2}/(16\tau_2)} + 2(8kp+2)pC_1^2\exp(-n/2) \\
+\ & (8kp+2)p(2C^*)^{1/2}\exp\{-n(1-(k/n)^{1/2})^2/16\} + 2(8kp+2)pC_1^2\exp[-n\{1-(k/n)^{1/2}\}^2/8],
\end{aligned}
$$

where $\tau_1 := \lambda_{\min}(\Sigma_0)$, $\tau_2 := \lambda_{\max}(\Sigma_0)$, $z = 4\tau_2(1+k/n+2(k/n)^{1/2})$, and $C^* = 8||A_n||^4/(n+\nu-2p+k-1)^4+z^4/4+64(8\tau_2 z^3/n+3(8\tau_2)^2z^2/n^2+6z(8\tau_2)^3/n^3+6(8\tau_2)^4/n^4)\exp\{-nz/(8\tau_2)\}$.

By applying $C_1$ and $C_2$ to $U_1(\cdot)$, we obtain an upper bound as

$$U_1(n,p,k,||A_n||,\nu_n) + U_2(n,p,k,||A_n||,\lambda_{\max}(\Sigma_0),\lambda_{min}(\Sigma_0),\nu_n).$$

If $k, \log p, ||A_n||, (\nu_n - 2p) = o(n)$ and $\lambda_{\max}(\Sigma_0)$ and $\lambda_{\min}(\Sigma_0)$ are constants, then

$$u_1 + u_2 = C\frac{k+\log p}{n} + o\Big(\frac{k+\log p}{n}\Big),$$

where $C = 2^{10}\log 5\{(2||\Sigma_0||)^{1/2} \vee 8||\Sigma_0||\}^3/||\Sigma_0^{-1}||$.

**Lemma 4.11** *Let the prior $\pi^i$ of $\Sigma_n$ be $IW_p(A_n,\nu_n)$. If $\nu_n - 2p = o(n)$ and $||T_{2k}(A_n)||^2 = o(n)$, then for $n \geq 4\log p||\Sigma_0||^{1/2}/\lambda_{\min}(\Sigma_0)$,*

$$\sup_{\Sigma_0\in\mathcal{B}_{p,k}} E_{\Sigma_0}\{E^{\pi^i}(||T_{2k}(\Sigma)-\Sigma_0||^2 \mid \mathbb{X}_n)\} \leq C\frac{k+\log p}{n} + o\Big(\frac{k+\log p}{n}\Big)$$

*where $C = [2^{11}\log 5\{(2||\Sigma_0||)^{1/2} \vee 8||\Sigma_0||\}^3/||\Sigma_0^{-1}||] \vee 2^6 3^2||\Sigma_0||$.*

**Proof** Since

$$E_{\Sigma_0}\{E^{\pi^i}(||T_{2k}(\Sigma)-\Sigma_0||^2 \mid \mathbb{X}_n)\} \leq 2E_{\Sigma_0}\{E^{\pi^i}(||T_{2k}(\Sigma)-T_{2k}(\hat\Sigma)||^2 \mid \mathbb{X}_n)\} + 2E_{\Sigma_0}(||T_{2k}(\hat\Sigma)-\Sigma_0||^2)$$

and

$$\begin{aligned} E_{\Sigma_0}(||T_{2k}(\hat\Sigma)-\Sigma_0||^2) \leq\ & 2E_{\Sigma_0}[||\frac{n}{n+\nu_n-2p+k-1}\{T_{2k}(S_n)-\Sigma_0\}||^2] \\ & +2||\frac{1}{n+\nu_n-2p+k-1}T_{2k}(A_n) - \frac{\nu_n-2p+k-1}{n+\nu_n-2p+k-1}\Sigma_0||^2, \end{aligned}$$

we have the following bound of the P-risk

$$\begin{aligned} E_{\Sigma_0}\{E^{\pi^i}(||T_{2k}(\Sigma)-\Sigma_0||^2 \mid \mathbb{X}_n)\} \leq\ & 2E_{\Sigma_0}\{E^{\pi^i}(||T_{2k}(\Sigma)-T_{2k}(\hat\Sigma)||^2 \mid \mathbb{X}_n)\} & (6)\\ & +4E_{\Sigma_0}\Big(||\frac{n}{n+\nu_n-2p+k-1}(T_{2k}(S_n)-\Sigma_0)||^2\Big) & (7)\\ & +8||\frac{1}{n+\nu_n-2p+k-1}T_{2k}(A_n)||^2 & (8)\\ & +8||\frac{\nu_n-2p+k-1}{n+\nu_n-2p+k-1}\Sigma_0||^2. & (9) \end{aligned}$$

First, we calculate the upper bound of (9). Since $\nu_n - 2p = o(n^{1/2})$ and $k = o(n)$,

$$
\begin{aligned}
||\frac{\nu_n - 2p + k - 1}{n + \nu_n - 2p + k - 1}\Sigma_0||^2 &\leq M_0^2 \frac{(k + \nu_n - 2p)^2}{n^2} \\
&\leq 4M_0^2 \Big\{\frac{\max(\nu_n - 2p, k)}{n}\Big\}^2.
\end{aligned}
$$

The term (8) is bounded by

$$
||\frac{1}{n + \nu_n - 2p + k - 1} T_{2k}(A_n)||^2 \leq \frac{||T_{2k}(A_n)||^2}{n^2}.
$$

The term (7) is bounded by

$$
\begin{aligned}
E_{\Sigma_0}\Big(||(T_{2k}(S_n) - \Sigma_0)||^2\Big) &\leq E_{\Sigma_0}(||T_{2k}(S_n) - ET_{2k}(S_n)||^2) \\
&\leq 9\{x^2 + E_{\Sigma_0}(||N^{(2k)}||^2 I(||N^{(2k)}|| > x)\} \\
&\leq 9\{x^2 + \int_x^\infty upr(||N^{(2k)}|| > u)du\} \\
&\leq 9\{x^2 + 2p\int_x^\infty u\exp(-nu^2/(8||\Sigma_0||))du \\
&\leq 9\{x^2 + 2p\exp\Big(-\frac{nx^2}{8||\Sigma_0||}\Big)\Big\{\frac{8||\Sigma_0||}{n} + \Big(\frac{8||\Sigma_0||}{n}\Big)^2\Big\},
\end{aligned}
$$

when $x \leq \lambda_{\min}(\Sigma_0)$, where $N^{(2k)} = \max_{1\leq l\leq p-2k+1} ||M_l^{*(2k)}(S_n) - EM_l^{*(2k)}(S_n)||$. The fourth inequality follows from the fact that $nv^T S_n v \sim v^T \Sigma_0 v \chi_n^2$. We set $x^2 = 16||\Sigma_0||\log p/n$, then for $\log p/n \leq \lambda_{\min}(\Sigma_0)/(4||\Sigma_0||^{1/2})$ obtain

$$
E_{\Sigma_0}\Big(||(T_{2k}(S_n) - \Sigma_0)||^2\Big) \leq 9\{16\frac{||\Sigma_0||\log p}{n} + \frac{2}{p}\Big\{\frac{8||\Sigma_0||}{n} + \Big(\frac{8||\Sigma_0||}{n}\Big)^2\Big\}.
$$

We only need to focus on the upper bound of (6) to get the desired result. Using Lemma 1 in Cai and Zhou (2012), the tapering transformation can be expressed as

$$
T_k(\Sigma) = (k/2)^{-1}\{S^{*(k)}(\Sigma) - S^{*(k/2)}(\Sigma)\},
$$

where $M_l^{*(m)}(\Sigma) = (\sigma_{ij} I\{l \leq i < l + m, l \leq j < l + m\})$ and $S^{*(m)}(\Sigma) = \sum_{l=1-m}^{p} M_l^{*(m)}(\Sigma)$. Thus, we can bound the $L_{p,p}$-norm of the tapered matrix as

$$
||T_k(\Sigma)||_p \leq (2/k)\Big[||S^{*(k)}(\Sigma)||_p + ||S^{*(k/2)}(\Sigma)||_p\Big].
$$

Also it satisfies that

$$
\begin{aligned}
||S^{*(m)}(\Sigma)||_p &\le \sum_{l=1}^{m} \Bigg|\Bigg| \sum_{-1\le j<p/m-1} M^{*(m)}_{jm+l}(\Sigma) \Bigg|\Bigg|_p \\
&\le m \max_{1\le l\le m} \Bigg|\Bigg| \sum_{-1\le j<p/m-1} M^{*(m)}_{jm+l}(\Sigma) \Bigg|\Bigg|_p \\
&\le m \max_{1-m\le l\le p} ||M^{*(m)}_{l}(\Sigma)||_p.
\end{aligned}
$$

Applying $k$ and $k/2$ instead of $m$, we obtain

$$
\begin{aligned}
||S^{*(k)}(\Sigma)||_p &\le k \max_{1-k\le l\le p} ||M^{*(k)}_{l}(\Sigma)||_p \\
||S^{*(k/2)}(\Sigma)||_p &\le (k/2) \max_{1-k/2\le l\le p} ||M^{*(k/2)}_{l}(\Sigma)||_p.
\end{aligned}
$$

Since the nonzero elements of $M^{*(k/2)}_l(\Sigma)$ are part of nonzero elements of $M^{*(k)}_r(\Sigma)$ for some $r$,

$$
\max_{1-k/2\le l\le p} ||M^{*(k/2)}_{l}(\Sigma)||_p \le \max_{1-k\le l\le p} ||M^{*(k)}_{l}(\Sigma)||_p.
$$

Therefore, the upper bound for the tapered matrix $T_k(\Sigma)$ is

$$
||T_k(\Sigma)||_p \le 3 \max_{1-k\le l\le p} ||M^{*(k)}_{l}(\Sigma)||_p = 3 \max_{1\le l\le p-k+1} ||M^{(k)}_{l}(\Sigma)||_p. \tag{10}
$$

Thus, we have the upper bound of (6),

$$
\begin{aligned}
E_{\Sigma_0}\{E^{\pi^i}(||T_{2k}(\Sigma-\hat{\Sigma})||_2^2 \mid \mathbb{X}_n)\} &\le 3E_{\Sigma_0}\{E^{\pi^i}(\max_{1\le l\le p-2k+1} ||M^{(2k)}_{l}(\Sigma-\hat{\Sigma})||^2 \mid \mathbb{X}_n)\} \\
&\le C\frac{k+\log p}{n} + o\Big(\frac{k+\log p}{n}\Big),
\end{aligned}
$$

where $C = 2^{11}\log 5\{(2||\Sigma_0||)^{1/2} \vee 8||\Sigma_0||\}^3/||\Sigma_0^{-1}||$. Collecting the bounds of (6), (7), (8) and (9), we complete the proof.

**Lemma 4.12** *The upper bound of P-risk minimax rate of the banding post-processed posterior (2) is*

$$
E_{\Sigma_0}\{E^{\pi^i}(||B^{(\epsilon_n)}_k(\Sigma)-\Sigma_0||^2 \mid \mathbb{X}_n)\} \le 6E_{\Sigma_0}\{E^{\pi^i}(||B_k(\Sigma)-\Sigma_0||^2 \mid \mathbb{X}_n)\} + 4\epsilon_n^2.
$$

**Proof** Taking $A = \Sigma_0$ and $B = B_k(\Sigma) - \Sigma_0$ in Lemma 4.14, we get

$$\begin{aligned}\lambda_{\min}\{B_k(\Sigma)\} &= \lambda_{\min}\{B_k(\Sigma) - \Sigma_0 + \Sigma_0\} \\ &\geq \lambda_{\min}(\Sigma_0) - ||B_k(\Sigma) - \Sigma_0||.\end{aligned}$$

This implies

$$0 \leq -\lambda_{\min}\{B_k(\Sigma)\} I(\lambda_{\min}\{B_k(\Sigma)\} < 0) \leq ||B_k(\Sigma) - \Sigma_0||.$$

Using the above inequality, we have

$$\begin{aligned}E_{\Sigma_0}\{E^{\pi^i}(||B_k^{\epsilon_n}(\Sigma) - \Sigma_0||^2|\mathbb{X}_n)\} &\leq 2E_{\Sigma_0}\{E^{\pi^i}(||B_k(\Sigma) - \Sigma_0||^2|\mathbb{X}_n)\} \\ &\quad +2E_{\Sigma_0}\{E^{\pi^i}([\epsilon_n - \lambda_{\min}(B_k(\Sigma))I\{\lambda_{\min}(B_k(\Sigma)) < 0\}]^2)\} \\ &\leq 2E_{\Sigma_0}E^{\pi^i}\Big[||B_k(\Sigma) - \Sigma_0||^2|\mathbb{X}_n\Big] + 4\epsilon_n^2 \\ &+ 4E_{\Sigma_0}[E^{\pi^i}\{(\lambda_{\min}\{B_k(\Sigma)\}I[\lambda_{\min}\{B_k(\Sigma)\} < 0])^2\}] \\ &\leq 6E_{\Sigma_0}\{E^{\pi^i}(||B_k(\Sigma) - \Sigma_0||^2|\mathbb{X}_n)\} + 4\epsilon_n^2.\end{aligned}$$

**Lemma 4.13** *Let the prior $\pi^i$ of $\Sigma_n$ be $IW_p(A_n, \nu_n)$. If $\nu_n - 2p = o(n)$ and $||T_{2k}(A_n)||^2 = o(n)$, then for $n \geq 4 \log p ||\Sigma_0||^{1/2}/\lambda_{\min}(\Sigma_0)$,*

$$\begin{aligned}\sup_{\Sigma_0 \in \mathcal{F}_\alpha} E_{\Sigma_0}\{E^{\pi^i}(||T_{2k}(\Sigma) - \Sigma_0||^2 \mid \mathbb{X}_n)\} &\leq C \min\left\{(\log k)^2 \frac{\log p + k}{n} + k^{-2\alpha}, \frac{p}{n}\right\} \\ &\quad + o\Big[\min\left\{(\log k)^2 \frac{\log p + k}{n} + k^{-2\alpha}, \frac{p}{n}\right\}\Big],\end{aligned}$$

*where $C = [2^{11} \log 5\{(2||\Sigma_0||)^{1/2} \vee 8||\Sigma_0||\}^3/||\Sigma_0^{-1}||] \vee 2^6 3^2||\Sigma_0|| \vee 4M^2 2^{-2\alpha} \vee 1$.*

**Proof** First we will show that when $p \geq n^{1/(2\alpha+1)}$

$$\sup_{\Sigma_0 \in \mathcal{F}_\alpha} E_{\Sigma_0}\{E^{\pi^i}(||T_{2k}(\Sigma) - \Sigma_0||^2 \mid \mathbb{X}_n)\} \leq C\Big(n^{-2\alpha/(2\alpha+1)} + \frac{\log p}{n}\Big) \qquad (11)$$

By the similar arguments used in proof of Lemma 4.11,

$$
\begin{aligned}
& E_{\Sigma_0}\{E^{\pi^i}(||T_{2k}(\Sigma) - \Sigma_0||^2 \mid \mathbb{X}_n)\} \\
\leq\ & 2E_{\Sigma_0}\{E^{\pi^i}(||T_{2k}(\Sigma) - T_{2k}(\hat{\Sigma})||^2 \mid \mathbb{X}_n)\} && (12)\\
+\ & 4E_{\Sigma_0}\Big[||\frac{n}{n+\nu_n-2p+k-1}\{T_{2k}(S_n) - E_{\Sigma_0}T_{2k}(S_n)\}||^2\Big] && (13)\\
+\ & 8||\frac{1}{n+\nu_n-2p+k-1}T_{2k}(A_n)||^2 && (14)\\
+\ & 8||\frac{\nu_n-2p+k-1}{n+\nu_n-2p+k-1}\Sigma_0||^2 && (15)\\
+\ & 4||\Sigma_0 - E_{\Sigma_0}T_{2k}(S_n)||^2. && (16)
\end{aligned}
$$

Using the inequality (6), (7), (8) and (9) in Lemma 4.11, the term (12), (13), (14) and (15) is bounded by $U(n, p, k, \nu_n, ||A_n||, \lambda_{\max}(\Sigma_0), \lambda_{\min}(\Sigma_0))$, which is defined in Lemma 4.11. The term (16) is bounded by $M^2(2k)^{-2\alpha}$. If we choose $k = n^{1/(2\alpha+1)}$, it gives the desired result (11).

For the case $p < n^{1/(2\alpha+1)}$, using Theorem 3.2 in Lee and Lee (2018) we can obtain

$$\sup_{\Sigma_0\in\mathcal{F}_\alpha} E_{\Sigma_0}\{E^{\pi^i}(||T_{2k}(\Sigma) - \Sigma_0||^2 \mid \mathbb{X}_n)\} \leq \frac{p}{n}.$$

**Lemma 4.14** *Let $A$ and $B$ be symmetric matrices. Then,*

$$\lambda_{\min}(A+B) + ||B|| \geq \lambda_{\min}(A).$$

**Proof** By the fact that $||B|| = \sup_{v:||v||=1} |v'Bv|$, $\min_{v:||v||=1} v'Bv + ||B|| \geq 0$, we have

$$
\begin{aligned}
\lambda_{\min}(A+B) + ||B|| &= \min_{v:||v||=1} v'(A+B)v + ||B|| \\
&\geq \min_{v:||v||=1} v'Ab + \min_{v:||v||=1} v'Bv + ||B|| \\
&\geq \min_{v:||v||=1} v'Ab = \lambda_{\min}(A).
\end{aligned}
$$

**Proof of Theorem 3.1** By (14) in Bhatia (2000), for any matrix $A$

$$||B_k(A)|| \leq \Big\{\log k + \log\pi + \frac{2}{\pi}(1+\frac{1}{2k})\Big\}||A||.$$

By applying this inequality to $T_{2k}(\Sigma) - \Sigma_0$, we can obtain

$$
\begin{aligned}
||B_k(\Sigma) - \Sigma_0|| &= ||B_k(T_{2k}(\Sigma) - \Sigma_0)|| \\
&\leq \Big\{\log k + \log\pi + \frac{2}{\pi}(1+\frac{1}{2k})\Big\}||T_{2k}(\Sigma) - \Sigma_0||.
\end{aligned}
$$

Applying Lemmas 4.11 and 4.12,

$$\sup_{\Sigma_0 \in \mathcal{B}_{p,k}} E_{\Sigma_0}\{E^{\pi^i}(||B_k^{(\epsilon_n)}(\Sigma) - \Sigma_0||^2 \mid \mathbb{X}_n)\} \leq 6C(\log k)^2 \frac{k + \log p}{n} + 4\epsilon_n^2,$$

where $C = 2^{11} \log 5\{(2||\Sigma_0||)^{1/2} \vee 8||\Sigma_0||\}^3/||\Sigma_0^{-1}||$.

The result and the proof of Theorem 3.2 are almost the same as Cai and Zhou (2010) and the only difference lies in the parameter spaces. We still give the proof below for the completeness of the paper.

**Proof of Theorem 3.2** Define a $p \times p$ matrix $B(m, k/2) = (b_{ij})$ as

$$b_{ij} = I(i = m \text{ and } m + 1 \leq j \leq k, \text{ or } j = m \text{ and } m + 1 \leq i \leq k)$$

and a subset of parameter space $\mathcal{B}_1$ as

$$\mathcal{B}_1 = \Big\{\Sigma(\theta) : \Sigma(\theta) = \epsilon I_p + \tau \sum_{m=1}^{k_h} \theta_m B(m, k_h), \theta = (\theta_m) \in \{0, 1\}^{k_h}\Big\},$$

where $\epsilon = (M_0 + M_1)/2$, $k_h = k/2$ and $\tau > 0$.

Note $\Sigma \in \mathcal{B}_1$ has k-band structure. Since for any $\Sigma \in \mathcal{B}_1$,

$$\lambda_{\max}(\Sigma) \leq \epsilon||I_p|| + \tau||\sum_{m=1}^{k_h} \theta_m B(m, k_h)|| \leq \epsilon + \tau k$$

$$\lambda_{\min}(\Sigma) \geq \lambda_{\min}(\epsilon I_p) - \tau||\sum_{m=1}^{k_h} \theta_m B(m, k_h)|| \geq \epsilon - \tau k,$$

for sufficiently small $\tau > 0$, $\lambda_{\max}(\Sigma) \leq M_0$ and $\lambda_{\min}(\Sigma) \geq M_1$; thus, $\mathcal{B}_1 \subset \mathcal{B}_{p,k}$.

Define another subset $\mathcal{B}_2$ as

$$\mathcal{B}_2 = \Big\{\Sigma_m : \Sigma_m = M_1 I_p + \Big\{(\frac{\eta}{n} \log p_1)^{1/2} I\{i = j = m\}\Big\}, 0 \leq m \leq p_1\Big\},$$

where $p_1 = \min\{p, e^{n/2}\}$ and $0 < \eta < \min\{(M_0 - M_1)^2, 1\}$. For any $\Sigma \in \mathcal{B}_1$, $\lambda_{\max}(\Sigma) \leq M_0$, and $\lambda_{\min}(\Sigma) \geq M_1$; thus, $\mathcal{B}_1 \cup \mathcal{B}_2 \subset \mathcal{B}_{p,k}$.

Using the proof of Lemma 7 of Cai and Zhou (2010),

$$\begin{aligned} \inf_{\hat{\Sigma}} \sup_{\mathcal{B}_2} E(||\hat{\Sigma} - \Sigma||^2) &\geq \frac{\eta \log p_1}{2n}\Big\{1 - \frac{1}{2p_1^{1/2}}\Big(\Big[1 - \Big\{1 - M_1 - \Big(\frac{\eta}{n}\log p_1\Big)^{1/2}\Big\}^2\Big]^{-n/2} - 1\Big)^{1/2}\Big\} \\ &:= L_1(n, p, M_0, M_1), \qquad (17) \end{aligned}$$

for $\eta \log p_1/n < 1/2$. If $M_0$ and $M_1$ are constants and $\log p = o(n)$, then $L_1(n, p, M_0, M_1) \asymp \log p/n$ . We now apply the Assouad lemma (Assouad; 1983) to get a lower bound of the minimax risk on the parameter space $\mathcal{B}_1$. Applying the Assouad lemma, we obtain

$$\inf_{\hat{\Sigma}} \max_{\theta \in \{0,1\}^{k_h}} 2^2 E_\theta ||\hat{\Sigma} - \Sigma(\theta)||^2 \geq \min_{H(\theta,\theta')\geq 1} \frac{||\Sigma(\theta) - \Sigma(\theta')||^2}{H(\theta, \theta')} \frac{k_h}{2} \min_{H(\theta,\theta')=1} ||P_\theta \wedge P_{\theta'}||,$$

where $\Sigma(\theta)$ is an element of $\mathcal{B}_1$. For the first factor in the lower bound, we use the similar technique used in the proof of Lemma 5 in Cai and Zhou (2010):

$$\begin{aligned}
\min_{H(\theta,\theta')\geq 1} \frac{||\Sigma(\theta) - \Sigma(\theta')||^2}{H(\theta, \theta')} &\geq \min_{H(\theta,\theta')\geq 1} \frac{||(\Sigma(\theta) - \Sigma(\theta'))v||^2}{||v||^2 H(\theta, \theta')} \\
&\geq \min_{H(\theta,\theta')\geq 1} \frac{H(\theta, \theta')(\tau k_h)^2}{k_h H(\theta, \theta')} \\
&\geq k_h \tau^2.
\end{aligned}$$

For the third factor in the lower bound, we will show that the following inequality holds for some constant $c_1 > 0$:

$$\min_{H(\theta,\theta')=1} ||P_\theta \wedge P_{\theta'}|| \geq c_1.$$

Note that for any $H(\theta, \theta') = 1$,

$$\begin{aligned}
||P_\theta \wedge P_{\theta'}|| &= 1 - ||P_\theta - P_{\theta'}||_1/2 \\
&\geq 1 - \{KL(P_{\theta'}||P_\theta)/2\}^{1/2} \\
&\geq 1 - \Big(n\Big[\frac{1}{2} tr\{\Sigma(\theta')\Sigma^{-1}(\theta)\} - \frac{1}{2}\log\det\{\Sigma(\theta')\Sigma^{-1}(\theta)\} - \frac{p}{2}\Big]/2\Big)^{1/2}.
\end{aligned}$$

Let $\Sigma(\theta') = D_1 + \Sigma(\theta)$ and $\lambda_i$ be the eigenvalues of $D_1\Sigma^{-1}(\theta)$. Then, $\lambda_i$'s are non-negative

since $D_1\Sigma^{-1}(\theta)$ is similar to $\Sigma^{-1/2}(\theta)D_1\Sigma^{-1/2}(\theta)$. It satisfies that

$$\begin{aligned}
\log\det\{\Sigma(\theta')\Sigma^{-1}(\theta)\} &= \log\det\{I_p + D_1\Sigma^{-1}(\theta)\} \\
&= \sum_{i=1}^{p}\lambda_i + \sum_{i=1}^{p}\{\log(1+\lambda_i) - \lambda_i\} \\
&\geq tr\{D_1\Sigma^{-1}(\theta)\} + \sum_{i=1}^{p}(\frac{\lambda_i}{\lambda_i+1} - \lambda_i) \\
&\geq tr\{D_1\Sigma^{-1}(\theta)\} - \sum_{i=1}^{p}\lambda_i^2 \\
&\geq tr\{D_1\Sigma^{-1}(\theta)\} - ||\Sigma^{-1}(\theta)||^2||D_1||_F^2 \\
&\geq tr\{D_1\Sigma^{-1}(\theta)\} - \frac{2k\tau^2}{(\epsilon-\tau k)^2}.
\end{aligned}$$

By letting $\tau^2 = \epsilon^2/(2nk)$

$$\begin{aligned}
n\Big[\frac{1}{2}tr\{\Sigma(\theta')\Sigma^{-1}(\theta)\} - \frac{1}{2}\log\det\{\Sigma(\theta')\Sigma^{-1}(\theta)\} - \frac{p}{2}\Big] &\leq \frac{nk\tau^2}{(\epsilon-\tau k)^2} \\
&= \frac{1}{2(1-\{k/(2n)\}^{1/2})}, \quad (18)
\end{aligned}$$

which implies

$$\begin{aligned}
4\inf_{\hat\Sigma}\sup_{\mathcal{B}_1} E(||\hat\Sigma - \Sigma||^2) &\geq \inf_{\hat\Sigma}\max_{\theta\in\{0,1\}^{k_h}} 2^2 E_\theta(||\hat\Sigma - \Sigma(\theta)||^2) \\
&\geq \left(1 - \frac{1}{2(1-(k/(2n))^{1/2})^{1/2}}\right)k_h^2\tau^2/2, \quad (19)
\end{aligned}$$

which is asymptotically same rate with $k/n$, if $k = o(n)$. Thus, we have the desired lower bound

$$\inf_{\hat\Sigma}\sup_{\mathcal{B}_1\cup\mathcal{B}_2}(E||\hat\Sigma - \Sigma||^2) \geq L(n,p,k,M_0,M_1),$$

where $L(n,p,k,M_0,M_1) \asymp (\log p + k)/n$, if $\log p, k = o(n)$, and $M_0$ and $M_1$ are constants. By Jensen's inequality

$$\inf_{(\pi,f)\in\Pi^*}\sup_{\Sigma_0\in\mathcal{B}_{p,k}} E_{\Sigma_0}\{E^\pi(||f(\Sigma) - \Sigma_0||^2 \mid \mathbb{X}_n)\} \geq \inf_{\hat\Sigma}\sup_{\Sigma_0\in\mathcal{B}_{p,k}} E(||\hat\Sigma - \Sigma_0||^2).$$

This completes the proof.

**Proof of Theorem 3.3** Let $\mathbb{X}_n$ be the random variable on an event space $(\Omega, \mathcal{F}, \mathbb{P})$. For $w \in \Omega$, define $R^{PPP,0}_{1-\alpha,n}(w)$, $R^{PPP}_{1-\alpha,n}(w)$ and $A_{1-\alpha}$ by the highest posterior density regions of $[n^{1/2}(\theta_1(\Sigma) - \hat{\theta}^*_1) \mid \mathbb{X}_n(w)]_{PPP,0}$, $[n^{1/2}(\theta_1(\Sigma) - \hat{\theta}^*_1) \mid \mathbb{X}_n(w)]_{PPP}$ and $N[0, \mathcal{I}^{-1}_{11\cdot 2}\{\theta_1(\Sigma_0), 0\}]$, respectively. By the definition, $n^{1/2}(C_{1-\alpha,n}(w) - \hat{\theta}^*_1) = R^{PPP}_{1-\alpha,n}(w)$ is satisfied , where $A + b = \{a + b : a \in A\}$ for any $A \subset \mathbb{R}^{p^*}$ and $b \in \mathbb{R}^{p^*}$. Also, let $\Pi^{PPP,0}$, $\Pi^{PPP}$ and $\Pi^C$ denote the probability measures of $[\Sigma \mid \mathbb{X}_n]_{PPP,0}$, $[\Sigma \mid \mathbb{X}_n]_{PPP}$ and $[\Sigma \mid \mathbb{X}_n]_C$, respectively.

Let $O_n := \{\Sigma : \lambda_{\min}(\Sigma) > \epsilon_n\}$. Then, by the definition of the banding post-process function with positive adjustment,

$$
\begin{aligned}
[n^{1/2}(\theta_1(\Sigma) - \hat{\theta}^*_1) \mid \mathbb{X}_n(w), \Sigma \in O_n]_{PPP,0} &\overset{d}{\equiv} [n^{1/2}(\theta_1(\Sigma) - \hat{\theta}^*_1) \mid \mathbb{X}_n(w), \Sigma \in O_n]_{PPP}, \quad (20)\\
\Pi^{PPP,0}(O_n^c \mid \mathbb{X}_n(w)) &= \Pi^{PPP}(O_n^c \mid \mathbb{X}_n(w)) := \eta_n(w).
\end{aligned}
$$

Define $R^{PPP}_{1-\alpha,n}(w)^{(O)}$ and $R^{PPP}_{1-\alpha,n}(w)^{(I)}$ as the highest posterior density regions of $[n^{1/2}(\theta_1(\Sigma) - \hat{\theta}^*_1) \mid \mathbb{X}_n(w), \Sigma \in O_n]_{PPP}$ and $[n^{1/2}(\theta_1(\Sigma) - \hat{\theta}^*_1) \mid \mathbb{X}_n(w), \Sigma \in O_n^c]_{PPP}$, respectively. Then, there exist $\alpha_1$ and $\beta_1$ such that

$$
R^{PPP}_{1-\alpha,n}(w) = R^{PPP}_{1-\alpha_1,n}(w)^{(O)} \cup R^{PPP}_{1-\beta_1,n}(w)^{(I)},
$$

where

$$
\frac{1 - \alpha - \eta_n(w)}{1 - \eta_n(w)} \le 1 - \alpha_1 \le \frac{1 - \alpha}{1 - \eta_n(w)}. \quad (21)
$$

Likewise, we define $(\alpha_2, \beta_2)$, $(\alpha_3, \beta_3)$, $R^{PPP,0}_{1-\alpha_2,n}(w)^{(O)}$, $R^{PPP,0}_{1-\alpha_2,n}(w)^{(I)}$, $R^{PPP,0}_{1-\alpha_3,n}(w)^{(O)}$ and $R^{PPP,0}_{1-\beta_3,n}(w)^{(I)}$ such that

$$
\begin{aligned}
R^{PPP,0}_{1-\alpha+\eta_n(w),n}(w) &= R^{PPP,0}_{1-\alpha_2,n}(w)^{(O)} \cup R^{PPP,0}_{1-\beta_2,n}(w)^{(I)}\\
R^{PPP,0}_{1-\alpha-\eta_n(w),n}(w) &= R^{PPP,0}_{1-\alpha_3,n}(w)^{(O)} \cup R^{PPP,0}_{1-\beta_3,n}(w)^{(I)},
\end{aligned}
$$

where

$$
\frac{1 - \alpha}{1 - \eta_n(w)} \le 1 - \alpha_2 \le \frac{1 - \alpha + \eta_n(w)}{1 - \eta_n(w)} \quad (22)
$$

$$
\frac{1 - \alpha - 2\eta_n(w)}{1 - \eta_n(w)} \le 1 - \alpha_3 \le \frac{1 - \alpha - \eta_n(w)}{1 - \eta_n(w)}. \quad (23)
$$

By (20), $R^{PPP}_{1-\alpha_1,n}(w)^{(O)} = R^{PPP,0}_{1-\alpha_1,n}(w)^{(O)}$.

By the definition of $\eta_n(w)$, we have $\eta_n(w) \longrightarrow 0$ as $n \to \infty$. Then, for all large $n$,

$$\begin{aligned} 1-\alpha_3 &\leq \frac{1-\alpha-\eta_n(w)}{1-\eta_n(w)} \\ &\leq 1-\alpha_1, \\ 1-\alpha_2 &\geq \frac{1-\alpha}{1-\eta_n(w)} \\ &\geq 1-\alpha_1, \end{aligned}$$

by (21)-(23). Then,

$$R^{PPP,0}_{1-\alpha_3,n}(w)^{(O)} \subset R^{PPP}_{1-\alpha_1,n}(w)^{(O)} \subset R^{PPP,0}_{1-\alpha_2,n}(w)^{(O)}.$$

Using $R^{PPP}_{1-\alpha_1,n}(w)^{(O)} = R^{PPP}_{1-\alpha,n}(w) \cap n^{1/2}(O_n - \hat{\theta}^*_1)$, $R^{PPP,0}_{1-\alpha_2,n}(w)^{(O)} = R^{PPP,0}_{1-\alpha+\eta_n(w),n} \cap n^{1/2}(O_n - \hat{\theta}^*_1)$ and $R^{PPP,0}_{1-\alpha_3,n}(w)^{(O)} = R^{PPP,0}_{1-\alpha-\eta_n(w),n} \cap n^{1/2}(O_n - \hat{\theta}^*_1)$, we obtain

$$R^{PPP,0}_{1-\alpha-\eta_n(w),n} \cap n^{1/2}(O_n - \hat{\theta}^*_1) \subset R^{PPP}_{1-\alpha,n}(w) \cap n^{1/2}(O_n - \hat{\theta}^*_1) \subset R^{PPP,0}_{1-\alpha+\eta_n(w),n} \cap n^{1/2}(O_n - \hat{\theta}^*_1).$$

It implies

$$R^{PPP}_{1-\alpha,n} \triangle R^{PPP,0}_{1-\alpha,n} \quad \subset \quad n^{1/2}(O^c_n - \hat{\theta}^*_1) \cup (R^{PPP,0}_{1-\alpha+\eta_n(w),n} \setminus R^{PPP,0}_{1-\alpha-\eta_n(w),n}), \tag{24}$$

where $\triangle$ is the symmetric difference.

Let $p^*$ be the dimension of $\theta_1(\Sigma)$. Denote the density functions on $\mathbb{R}^{p^*}$ of $[n^{1/2}(\theta_1(\Sigma) - \hat{\theta}^*_1) \mid \mathbb{X}_n(w)]_{PPP,0}$, $[n^{1/2}(\theta_1(\Sigma) - \hat{\theta}_1) \mid \mathbb{X}_n(w)]_C$, $N[0, \mathcal{I}^{-1}_{11\cdot 2}\{\theta_1(\Sigma_0), 0\}]$ and $N[0, \mathcal{I}^{-1}_{11}\{\theta_1(\Sigma_0), 0\}]$ by $\pi^{PPP,0}_n(x; w)$, $\pi^C_n(x; w)$, $p^{PPP}(x)$ and $p^{PPP}_2(x)$, respectively.

Using (24), we obtain

$$\begin{aligned} \int_{R^{PPP}_{1-\alpha,n}(w) \triangle R^{PPP,0}_{1-\alpha,n}(w)} p^{PPP}(x)dx &\leq \int_{R^{PPP}_{1-\alpha,n}(w) \triangle R^{PPP,0}_{1-\alpha,n}(w)} \pi^{PPP,0}_n(x)dx \\ &\quad + \int_{R^{PPP}_{1-\alpha,n}(w) \triangle R^{PPP,0}_{1-\alpha,n}(w)} |(p^{PPP} - \pi^{PPP,0}_n)(x)|dx \\ &\leq 3\eta_n(w) + TV_1(w), \end{aligned}$$

which implies

$$m_1 \int_{(R^{PPP}_{1-\alpha,n}(w) \triangle R^{PPP,0}_{1-\alpha,n}(w)) \cap B_{M_1}} dx \quad \leq \quad 3\eta_n(w) + TV_1(w), \tag{25}$$

where $TV_1(w) := ||[n^{1/2}(\theta_1(\Sigma) - \hat{\theta}_1^*) \mid \mathbb{X}_n(w)]_{PPP,0} - N(0, \mathcal{I}_{11\cdot 2}^{-1}\{\theta_1(\Sigma_0), 0\})||_{TV}$, $B_{M_1} = \{x \in \mathbb{R}^{p^*} : ||x||_2 \leq M_1\}$ and $m_1 = \inf_{x \in B_{M_1}} p^{PPP}(x)$.

Define

$$U_{n,\delta_1}(w) := \{x \in \mathbb{R}^{p^*} : |\pi_n^{PPP,0}(x) - p^{PPP}(x)| > \delta_1\}$$

for a sufficiently small positive real number $\delta_1$. Then,

$$\begin{aligned} \delta_1 \int_{U_{n,\delta_1}(w)} dx &\leq \int_{U_{n,\delta_1}(w)} |\pi_n^{PPP,0}(x;w) - p^{PPP}(x)| dx \\ &\leq TV_1(w). \end{aligned} \tag{26}$$

Define

$$\begin{aligned} \xi_{n,\delta_1}(w) &:= \int_{U_{n,\delta_1}(w)} \pi_n^{PPP,0}(x) dx \vee \int_{U_{n,\delta_1}(w)} p^{PPP}(x) dx, \qquad (27) \\ A^{+}_{1-\alpha+\xi_{n,\delta_1}(w),\delta_1} &:= \{x \in \mathbb{R}^{p^*} : p^{PPP}(x) - \delta_1 \geq c^{+}_{1-\alpha}\}, \\ A^{++}_{1-\alpha+\xi_{n,\delta_1}(w),\delta_1} &:= \{x \in \mathbb{R}^{p^*} : p^{PPP}(x) + \delta_1 \geq c^{+}_{1-\alpha}\}, \\ A^{-}_{1-\alpha-\xi_{n,\delta_1}(w),\delta_1} &:= \{x \in \mathbb{R}^{p^*} : p^{PPP}(x) + \delta_1 \geq c^{-}_{1-\alpha}\}, \\ A^{--}_{1-\alpha-\xi_{n,\delta_1}(w),\delta_1} &:= \{x \in \mathbb{R}^{p^*} : p^{PPP}(x) - \delta_1 \geq c^{-}_{1-\alpha}\}, \end{aligned}$$

where $c^{+}_{1-\alpha}$ and $c^{-}_{1-\alpha}$ are constants such that

$$\int_{A^{+}_{1-\alpha+\xi_{n,\delta_1}(w),\delta_1}} (p^{PPP}(x) - \delta_1) dx = 1 - \alpha + \xi_{n,\delta_1}(w),$$
$$\int_{A^{-}_{1-\alpha-\xi_{n,\delta_1}(w),\delta_1}} (p^{PPP}(x) + \delta_1) dx = 1 - \alpha - \xi_{n,\delta_1}(w).$$

Then, we have

$$\begin{aligned} \int_{A^{+}_{1-\alpha+\xi_{n,\delta_1}(w),\delta_1} \setminus A^{-}_{1-\alpha-\xi_{n,\delta_1}(w),\delta_1}} p^{PPP}(x) dx &\leq m_2 \delta_1 + 2\xi_{n,\delta_1}(w), \\ \int_{A^{++}_{1-\alpha+\xi_{n,\delta_1}(w),\delta_1} \setminus A^{+}_{1-\alpha+\xi_{n,\delta_1}(w),\delta_1}} p^{PPP}(x) dx &\leq \int p^{PPP}(x) I(c^{+}_{1-\alpha} - \delta_1 < p^{PPP}(x) < c^{+}_{1-\alpha} + \delta_1) dx \\ &\leq h(\delta_1), \qquad (28) \\ \int_{A^{-}_{1-\alpha-\xi_{n,\delta_1}(w),\delta_1} \setminus A^{--}_{1-\alpha-\xi_{n,\delta_1}(w),\delta_1}} p^{PPP}(x) dx &\leq \int p^{PPP}(x) I(c^{-}_{1-\alpha} - \delta_1 < p^{PPP}(x) < c^{-}_{1-\alpha} + \delta_1) dx \\ &\leq h(\delta_1), \end{aligned}$$

for a positive constant $m_2$ and a real valued function $h(\delta_1)$, which converges to zero as $\delta_1 \longrightarrow 0$. Since

$$\begin{aligned}
\int \pi_n^{PPP,0} I(\pi_n^{PPP,0} > c_{1-\alpha}^{+})dx &\geq \int \pi_n^{PPP,0} I(\pi_n^{PPP,0} > c_{1-\alpha}^{+}) I(U_{n,\delta_1}(w)^c)dx \\
&\geq \int (p^{PPP} - \delta_1) I(p^{PPP} - \delta_1 > c_{1-\alpha}^{+}) I(U_{n,\delta_1}(w)^c)dx \\
&= 1 - \alpha + \xi_{n,\delta_1}(w) - \int (p^{PPP} - \delta_1) I(p^{PPP} - \delta_1 > c_{1-\alpha}^{+}) I(U_{n,\delta_1}(w))dx \\
&\geq 1 - \alpha + \xi_{n,\delta_1}(w) - \int p^{PPP} I(U_{n,\delta_1}(w))dx \\
&\geq 1 - \alpha,
\end{aligned}$$

we obtain

$$\begin{aligned}
R_{1-\alpha,n}^{PPP,0} \cap U_{n,\delta_1}(w)^c &\subset \{\pi_n^{PPP,0} > c_{1-\alpha}^{+}\} \cap U_{n,\delta_1}(w)^c \\
&\subset \{p^{PPP} + \delta_1 > c_{1-\alpha}^{+}\} \cap U_{n,\delta_1}(w)^c \\
&= A_{1-\alpha+\xi_{n,\delta_1}(w),\delta_1}^{++} \cap U_{n,\delta_1}(w)^c. \qquad (29)
\end{aligned}$$

Similarly, we have

$$\begin{aligned}
\int \pi_n^{PPP,0} I(\pi_n^{PPP,0} > c_{1-\alpha}^{-})dx &= \int \pi_n^{PPP,0} I(\pi_n^{PPP,0} > c_{1-\alpha}^{-})(I(U_{n,\delta_1}(w)) + I(U_{n,\delta_1}(w)^c))dx \\
&\leq \xi_{n,\delta_1}(w) + \int (p^{PPP}(x) + \delta_1) I(p^{PPP} + \delta_1 > c_{1-\alpha}^{-}) I(U_{n,\delta_1}(w)^c)dx \\
&\leq 1 - \alpha,
\end{aligned}$$

which implies

$$\begin{aligned}
R_{1-\alpha,n}^{PPP,0} \cap U_{n,\delta_1}(w)^c &\supset \{\pi_n^{PPP,0} > c_{1-\alpha}^{-}\} \cap U_{n,\delta_1}(w)^c \\
&\supset \{p^{PPP} - \delta_1 > c_{1-\alpha}^{-}\} \cap U_{n,\delta_1}(w)^c \\
&= A_{1-\alpha+\xi_{n,\delta_1}(w),\delta_1}^{--} \cap U_{n,\delta_1}(w)^c. \qquad (30)
\end{aligned}$$

Collecting (29) and (30), we obtain

$$A_{1-\alpha+\xi_{n,\delta_1}(w),\delta_1}^{--} \cap U_{n,\delta_1}(w)^c \subset R_{1-\alpha,n}^{PPP,0} \cap U_{n,\delta_1}(w)^c \subset A_{1-\alpha+\xi_{n,\delta_1}(w),\delta_1}^{++} \cap U_{n,\delta_1}(w)^c,$$

and it is obvious

$$A^{--}_{1-\alpha+\xi_{n,\delta_1}(w),\delta_1} \subset A_{1-\alpha} \subset A^{++}_{1-\alpha+\xi_{n,\delta_1}(w),\delta_1}.$$

Thus,

$$(R^{PPP,0}_{1-\alpha,n} \triangle A_{1-\alpha}) \cap U_{n,\delta_1}(w)^c \subset A^{++}_{1-\alpha+\xi_{n,\delta_1}(w),\delta_1} \setminus A^{--}_{1-\alpha+\xi_{n,\delta_1}(w),\delta_1}.$$

Let $M_2 = \sup_{x \in \mathbb{R}^{p^*}} p_2^{PPP}(x) \vee \sup_{x \in \mathbb{R}^{p^*}} p^{PPP}(x)$ and

$$TV_2(w) := ||[n^{1/2}(\theta_1(\Sigma) - \hat{\theta}_1^*) \mid \mathbb{X}_n(w)]_C - N(0, \mathcal{I}_{11}^{-1}\{\theta_1(\Sigma_0), 0\})||_{TV}.$$

For a sufficiently positive small number $\delta_2$, we obtain

$$\begin{aligned}
& |E_{\Sigma_0}(\Pi_n^C(n^{1/2}(\theta_1 - \hat{\theta}_1^*) \in R^{PPP}_{1-\alpha,n} \mid \mathbb{X}_n)) - E_{\Sigma_0}(\Pi_n^C(n^{1/2}(\theta_1 - \hat{\theta}_1^*) \in A_{1-\alpha} \mid \mathbb{X}_n))| \\
\leq\ & E_{\Sigma_0}\Big(2TV_2 + \Big|\int_{R^{PPP}_{1-\alpha,n}} p_2^{PPP}(x - n^{1/2}(\hat{\theta}_1 - \hat{\theta}_1^*))dx - \int_{A_{1-\alpha}} p_2^{PPP}(x - n^{1/2}(\hat{\theta}_1 - \hat{\theta}_1^*))dx\Big|\Big) \\
\leq\ & E_{\Sigma_0}\Big(2TV_2 + \int_{R^{PPP}_{1-\alpha,n} \triangle R^{PPP,0}_{1-\alpha,n}} p_2^{PPP}(x - n^{1/2}(\hat{\theta}_1 - \hat{\theta}_1^*))dx \\
& + \Big|\int_{R^{PPP,0}_{1-\alpha,n}} p_2^{PPP}(x - n^{1/2}(\hat{\theta}_1 - \hat{\theta}_1^*))dx - \int_{A_{1-\alpha}} p_2^{PPP}(x - n^{1/2}(\hat{\theta}_1 - \hat{\theta}_1^*))dx\Big|\Big) \\
\leq\ & E_{\Sigma_0}\Big(2TV_2 + \int_{R^{PPP}_{1-\alpha,n} \triangle R^{PPP,0}_{1-\alpha,n}} p_2^{PPP}(x - n^{1/2}(\hat{\theta}_1 - \hat{\theta}_1^*))dx \\
& + \int_{((R^{PPP,0}_{1-\alpha,n} \triangle A_{1-\alpha}) \cap U_{n,\delta_1}(w)^c) \cup U_{n,\delta_1}(w)} p_2^{PPP}(x - n^{1/2}(\hat{\theta}_1 - \hat{\theta}_1^*))dx\Big) \\
\leq\ & E_{\Sigma_0}\Big(2TV_2 + M_2 \int_{R^{PPP}_{1-\alpha,n} \triangle R^{PPP,0}_{1-\alpha,n} \cap B_{M_1}} dx + \int_{B^c_{M_1}} p_2^{PPP}(x - n^{1/2}(\hat{\theta}_1 - \hat{\theta}_1^*))dx \\
& + M_2 \int_{U_{n,\delta_1}(w)} dx + \int_{A^{++}_{1-\alpha+\delta_2,\delta_1} \setminus A^{--}_{1-\alpha-\delta_2,\delta_1}} p_2^{PPP}(x - n^{1/2}(\hat{\theta}_1 - \hat{\theta}_1^*))dx I(\xi_{n,\delta_1} \leq \delta_2) + I(\xi_{n,\delta_1} > \delta_2)\Big) \\
=\ & E_{\Sigma_0}\Big\{2TV_2 + M_2 \int_{R^{PPP}_{1-\alpha,n} \triangle R^{PPP,0}_{1-\alpha,n} \cap B_{M_1}} dx + M_2 \int_{U_{n,\delta_1}(w)} dx + I(\xi_{n,\delta_1} > \delta_2)\Big\} \qquad (31) \\
& + E_{\Sigma_0}\Big(E[I\{Z + n^{1/2}(\hat{\theta}_1 - \hat{\theta}_1^*) \in B^c_{M_1} \cup (A^{++}_{1-\alpha+\delta_2,\delta_1} \setminus A^{--}_{1-\alpha-\delta_2,\delta_1})\} \mid \mathbb{X}_n] I(\xi_{n,\delta_1} \leq \delta_2)\Big), \qquad (32)
\end{aligned}$$

where $[Z \mid \mathbb{X}_n] \sim N(0, [\mathcal{I}_{11}\{\theta_1(\Sigma_0), 0\}]^{-1})$.

Now we show that (31) and (32) converge to zero as $n \longrightarrow \infty$. By collecting (24)-(27),

an upper bound of (31) is given by

$$\begin{aligned} & E_{\Sigma_0}\Big(2TV_2 + (\frac{M_2}{m_1} + \frac{M_2}{\delta_1} + \frac{M_2+\delta_1}{\delta_1\delta_2})TV_1 + \frac{3M_2}{m_1}\eta_n\Big) \\ \longrightarrow\; & \frac{3M_2}{m_1}\lim_{n\longrightarrow\infty} E_{\Sigma_0}[\Pi^{PPP,0}\{\lambda_{\min}(\Sigma) < \epsilon_n \mid \mathbb{X}_n\}], \end{aligned}$$

as $n \longrightarrow \infty$. By Lemma 4.14 and the proof of Theorem 3.1,

$$\begin{aligned} E_{\Sigma_0}[\Pi^{PPP,0}\{\lambda_{\min}(\Sigma) < \epsilon_n \mid \mathbb{X}_n\}] &\le E_{\Sigma_0}(\Pi^{PPP,0}(\lambda_{\min}(\Sigma_0) - ||\Sigma(\theta_1,0) - \Sigma_0|| < \epsilon_n \mid \mathbb{X}_n)) \\ &\le \frac{E_{\Sigma_0}(E^{PPP,0}(||\Sigma(\theta_1,0)-\Sigma_0||^2))}{(\lambda_{\min}(\Sigma_0)-\epsilon_n)^2} \\ &\le c_2(\log k)^2\frac{k+\log p}{n(\lambda_{\min}(\Sigma_0)-\epsilon_n)^2}. \end{aligned}$$

Since the last term converges to zero $n \longrightarrow \infty$, it implies that (31) tends to zero as $n \longrightarrow \infty$. On the other hand, using Lemma 4.1 and the law of total variance, we obtain

$$\begin{aligned} \sqrt{n}\left[\hat{\theta}_1 - \hat{\theta}_1^*\right] &\xrightarrow{d} N(0, [\mathcal{I}_{11\cdot 2}\{\theta_1(\Sigma_0), 0\}]^{-1} - [\mathcal{I}_{11}\{\theta_1(\Sigma_0), 0\}]^{-1}), \\ \left[Z + n^{1/2}(\hat{\theta}_1 - \hat{\theta}_1^*)\right] &\xrightarrow{d} N(0, \mathcal{I}_{11\cdot 2}^{-1}(\theta_1(\Sigma_0), 0)), \end{aligned}$$

By the above result and the inequalities in (28), as $n \longrightarrow \infty$, (32) converges to

$$\begin{aligned} & \lim_{n\longrightarrow\infty} E_{\Sigma_0}(E[I\{Z + n^{1/2}(\hat{\theta}_1 - \hat{\theta}_1^*) \in B_{M_1}^c \cup (A_{1-\alpha+\delta_2,\delta_1}^{++} \setminus A_{1-\alpha-\delta_2,\delta_1}^{--})\} \mid \mathbb{X}_n]) \\ \le\; & m_2\delta_1 + 2\delta_2 + 2h(\delta_1) + \int_{B_{M_1}^c} p^{PPP}(x)dx, \end{aligned}$$

which goes to zero as $M_1 \longrightarrow \infty$, $\delta_1 \vee \delta_2 \longrightarrow 0$. Therefore, we obtain

$$\lim_{n\longrightarrow\infty} |E_{\Sigma_0}([n^{1/2}(\theta_1 - \hat{\theta}_1^*) \in R_{1-\alpha,n}^{PPP} \mid \mathbb{X}_n]_C) - E_{\Sigma_0}([n^{1/2}(\theta_1 - \hat{\theta}_1^*) \in A_{1-\alpha} \mid \mathbb{X}_n]_C)| = 0.$$

Since

$$E_{\Sigma_0}\Big([n^{1/2}(\theta_1 - \hat{\theta}_1^*) \in R_{1-\alpha,n}^{PPP} \mid \mathbb{X}_n]_C\Big) = E_{\Sigma_0}\Big([n^{1/2}(\theta_1 - \hat{\theta}_1^*) \in n^{1/2}(C_{1-\alpha,n} - \hat{\theta}_1^*) \mid \mathbb{X}_n]_C\Big),$$

and

$$\lim_{n\longrightarrow\infty} E_{\Sigma_0}([n^{1/2}(\theta_1 - \hat{\theta}_1^*) \in n^{1/2}(C_{1-\alpha,n} - \hat{\theta}_1^*) \mid \mathbb{X}_n]_C) = 1-\alpha,$$

we prove

$$\lim_{n\longrightarrow\infty} E_{\Sigma_0}([\theta_1 \in C_{1-\alpha,n} \mid \mathbb{X}_n]_C) = 1-\alpha.$$

**Proof of Theorem 1.1** Using Lemma 4.13, it can be shown similar with the proof of Theorem 3.1.

**Proof of Theorem 1.2** First consider the case $p \geq n^{1/(2\alpha+1)}$. Define a $p \times p$ matrix $B(m, k/2) = (b_{ij})$ as

$$b_{ij} = I(i = m \text{ and } m+1 \leq j \leq k, \text{ or } j = m \text{ and } m+1 \leq i \leq k)$$

and a subset of parameter space $\mathcal{B}_1$ as

$$\mathcal{B}_1 = \Big\{\Sigma(\theta) : \Sigma(\theta) = \epsilon I_p + \tau \sum_{m=1}^{k_h} \theta_m B(m, k_h), \theta = (\theta_m) \in \{0, 1\}^{k_h}\Big\},$$

where $\epsilon = (M_0 + M_1)/2$, $k_h = k/2$ and $\tau > 0$. Setting $k = n^{1/(2\alpha+1)}$ and $\tau^2 = (M \wedge \epsilon^2/2)/(nk)$, it satisfies that $\max_j\{\sum_i |\sigma_{ij}| : |i-j| > m\} \leq Mm^{-\alpha}$ for all $m$ and any $\Sigma \in \mathcal{B}_1$. Since for any $\Sigma \in \mathcal{B}_1$,

$$\lambda_{\max}(\Sigma) \leq \epsilon ||I_p|| + \tau || \sum_{m=1}^{k_h} \theta_m B(m, k_h)|| \leq \epsilon + \tau k$$

$$\lambda_{\min}(\Sigma) \geq \lambda_{\min}(\epsilon I_p) - \tau || \sum_{m=1}^{k_h} \theta_m B(m, k_h)|| \geq \epsilon - \tau k,$$

$\lambda_{\max}(\Sigma) \leq M_0$ and $\lambda_{\min}(\Sigma) \geq M_1$; thus, $\mathcal{B}_1 \subset \mathcal{F}_\alpha$.

Define another subset $\mathcal{B}_2$ as

$$\mathcal{B}_2 = \Big\{\Sigma_m : \Sigma_m = M_1 I_p + \Big\{\Big(\frac{\eta}{n}\log p_1\Big)^{1/2} I\{i = j = m\}\Big\}, 0 \leq m \leq p_1\Big\},$$

where $p_1 = \min\{p, e^{n/2}\}$ and $0 < \eta < \min\{(M_0 - M_1)^2, 1\}$. For any $\Sigma \in \mathcal{B}_2$, $\lambda_{\max}(\Sigma) \leq M_0$, and $\lambda_{\min}(\Sigma) \geq M_1$; thus, $\mathcal{B}_1 \cup \mathcal{B}_2 \subset \mathcal{F}_\alpha$.

By (17),

$$\inf_{\hat{\Sigma}} \sup_{\mathcal{B}_2} E(||\hat{\Sigma} - \Sigma||^2) \geq L_1(n, p, M_0, M_1),$$

for $\min(M_0 - M_1, 1) \log p/n < 1/2$. If $M_0$ and $M_1$ are constants and $\log p = o(n)$, then $L_1(n, p, M_0, M_1) \asymp \log p/n$ . Using inequality (19) and the fact that we set $k = n^{1/(2\alpha+1)}$

and $\tau^2 = (M \wedge \epsilon^2/2)/nk$,

$$
\begin{aligned}
4 \inf_{\hat{\Sigma}} \sup_{\mathcal{B}_1} E(||\hat{\Sigma} - \Sigma||^2) &\geq \left(1 - \frac{1}{2(1-(k/(2n))^{1/2})^{1/2}}\right) k_h^2 \tau^2/2 \\
&\geq (M \wedge \epsilon)\left(1 - \frac{1}{2(1-(n^{-2\alpha/(2\alpha+1)}/2)^{1/2})^{1/2}}\right) n^{-2\alpha/(2\alpha+1)}/16.
\end{aligned}
$$

The lower bounds of $\mathcal{B}_1$ and $\mathcal{B}_2$ lead to the following lower bound of $\mathcal{F}_\alpha$:

$$
\inf_{\hat{\Sigma}} \sup_{\mathcal{F}_\alpha} E(||\hat{\Sigma} - \Sigma||^2) \geq L(n, p, M, M_0, M_1, \alpha),
$$

which has rate of $n^{2\alpha/(2\alpha+1)} + \log p/n$, if $\log p = o(n)$, $n^{2\alpha/(2\alpha+1)} > 0.5$ and $M$, $M_0$, $M_1$, $\alpha$ are constants.

For the case $p < n^{1/(2\alpha+1)}$, define

$$
\mathcal{F}_* = \left\{\Sigma(\theta) : \Sigma(\theta) = \epsilon I_p + \tau^* \frac{1}{(np)^{1/2}} \sum_{m=1}^{p/2} \theta_m B(m, p/2), \theta = (\theta_m) \in \{0,1\}^{p/2}\right\}.
$$

By setting $\tau^{*2} = M \wedge \epsilon^2/2$, we have $\mathcal{F}_* \subset \mathcal{F}_\alpha$. Using the fact that $\mathcal{F}_*$ has same format with $\mathcal{B}_1$ and inequality (19), we obtain

$$
\begin{aligned}
4 \inf_{(\pi,f)\in\Pi^*} \sup_{\Sigma_0\in\mathcal{F}_*} E_{\Sigma_0}\{E^\pi(||f(\Sigma) - \Sigma_0||^2)\} &\geq 4 \inf_{\hat{\Sigma}} \sup_{\Sigma_0\in\mathcal{F}_*} E(||\hat{\Sigma} - \Sigma_0||^2) \\
&\geq \left(1 - \frac{1}{2(1-(k/(2n))^{1/2})^{1/2}}\right) k_h^2 \tau^{*2}/(2np) \\
&\geq (M \wedge \epsilon^2)\left(1 - \frac{1}{2(1-(p/(2n))^{1/2})^{1/2}}\right) \frac{p}{16n}.
\end{aligned}
$$

**Proof of Theorem 1.3** We use (14) in Bhatia (2000) as in the proof of Theorem 3.1.

$$
\begin{aligned}
||B_k(S_n) - \Sigma_0|| &= ||B_k(T_{2k}(S_n)) - \Sigma_0|| \\
&\leq ||B_k(T_{2k}(S_n) - \Sigma_0)|| + ||B_k(\Sigma_0) - \Sigma_0||
\end{aligned}
$$

Using the same technique as in the proof of Theorem 3.1, we obtain

$$
||\ B_k(T_{2k}(S_n) - \Sigma_0)\ || \leq C(n, p, k, \nu_n, ||A_n||, ||\Sigma_0||, \lambda_{\min}(\Sigma_0)) \log k ||T_{2k}(S_n) - \Sigma_0||.
$$

By the facts that $\Sigma \in \mathcal{F}_\alpha$ and the upper bound of the tapering estimator in Cai and Zhou (2010), the upper bound is obtained as

$$
\begin{aligned}
E(||B_k(S_n) - \Sigma_0||^2) &\leq 2C(n, p, k, \nu_n, ||A_n||, ||\Sigma_0||, \lambda_{\min}(\Sigma_0))^2 (\log k)^2 E(||T_{2k}(S_n) - \Sigma_0||^2) \\
&\quad + 2||B_k(\Sigma_0) - \Sigma_0||^2 \\
&\leq 2C(n, p, k, \nu_n, ||A_n||, ||\Sigma_0||, \lambda_{\min}(\Sigma_0))^2 (\log k)^2 \frac{\log p + k}{n} + 2M^2 k^{-2\alpha}.
\end{aligned}
$$

# References


Assouad, P. (1983). Deux remarques sur l'estimation, *Comptes rendus des séances de l'Académie des sciences. Série 1 Mathématique* **296**(23): 1021–1024.

Bhatia, R. (2000). Pinching, trimming, truncating, and averaging of matrices, *The American Mathematical Monthly* **107**(7): 602–608.

Bickel, P. J. and Levina, E. (2008). Regularized estimation of large covariance matrices, *The Annals of Statistics* pp. 199–227.

Cai, T. T. and Zhou, H. H. (2010). Optimal rates of convergence for covariance matrix estimation, *The Annals of Statistics* **38**(4): 2118–2144.

Cai, T. T. and Zhou, H. H. (2012). Minimax estimation of large covariance matrices under $\ell_1$-norm, *Statistica Sinica* pp. 1319–1349.

Du, X. and Ghosal, S. (2018). Bayesian discriminant analysis using a high dimensional predictor, *Sankhya A* **80**(1): 112–145.

Eldar, Y. C. and Kutyniok, G. (2012). *Compressed sensing: theory and applications*, Cambridge University Press.

Lee, K. (2018). *Asymptotic properties of posteriors for large covariance matrices*, PhD thesis, Seoul National University.

Lee, K. and Lee, J. (2018). Optimal Bayesian minimax rates for unconstrained large covariance matrices, *Bayesian Analysis* **13**(4): 1215–1233.

Liu, J., Zhong, L., Wickramasuriya, J. and Vasudevan, V. (2009). uWave: Accelerometer-based personalized gesture recognition and its applications, *Pervasive and Mobile Computing* **5**(6): 657–675.

Press, S. J. (2005). *Applied multivariate analysis: using Bayesian and frequentist methods of inference*, Courier Corporation.

Wainwright, M. J. (2019). *High-dimensional statistics: A non-asymptotic viewpoint*, Vol. 48, Cambridge University Press.
